# Supplementary material for: Origin of Unusual Composition of 3He-Rich Solar Energetic Particles
Source: arXiv:2510.17100 ancillary file (2025-10-20)
Supplement: Supplementary file 1 [file ApJ_published_version.pdf]

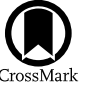

# Origin of the Unusual Composition of $^3\text{He}$ -rich Solar Energetic Particles

Radoslav Bučík<sup>1</sup> , Glenn M. Mason<sup>2</sup> , Sargam M. Mulay<sup>3</sup> , George C. Ho<sup>1</sup> , Robert F. Wimmer-Schweingruber<sup>4</sup> , andJavier Rodríguez-Pacheco<sup>5</sup> <sup>1</sup> Southwest Research Institute, San Antonio, TX 78238, USA; [radoslav.bucik@swri.org](mailto:radoslav.bucik@swri.org)<sup>2</sup> Applied Physics Laboratory, Johns Hopkins University, Laurel, MD 20723, USA<sup>3</sup> School of Physics and Astronomy, University of Glasgow, Glasgow, G12 8QQ, UK<sup>4</sup> Institut für Experimentelle und Angewandte Physik, Christian-Albrechts-Universität zu Kiel, 24118 Kiel, Germany<sup>5</sup> Universidad de Alcalá, Space Research Group, 28805 Alcalá de Henares, Spain

Received 2025 January 13; revised 2025 February 7; accepted 2025 February 8; published 2025 March 7

## Abstract

We examine  $^3\text{He}$ -rich solar energetic particles (SEPs) detected on 2023 October 24–25 by Solar Orbiter at 0.47 au. Measurements reveal that heavy-ion enhancements increase irregularly with mass, peaking at S, C, and especially N, Si, and S, stand out in the enhancement pattern with large abundances. Except for  $^3\text{He}$ , heavy-ion spectra can only be measured below  $0.5 \text{ MeV nucleon}^{-1}$ . At  $0.386 \text{ MeV nucleon}^{-1}$ , the event shows a huge  $^3\text{He}/^4\text{He}$  ratio of  $75.2 \pm 33.9$ , larger than previously observed. Solar Dynamics Observatory extreme-ultraviolet data show a minifilament eruption at the solar source of  $^3\text{He}$ -rich SEPs that triggered a straight tiny jet. Located at the boundary of a low-latitude coronal hole, the jet base is a bright, small-scale region with a supergranulation scale size. The emission measure (EM) provides relatively cold source temperatures of  $1.5\text{--}1.7 \text{ MK}$  between the filament eruption and nonthermal type III radio burst onset. Analysis suggests that the EM distribution of temperature in the solar source could be a factor that affects the preferential selection of heavy ions for heating or acceleration, thus shaping the observed enhancement pattern. Including previously reported similar events indicates that the eruption of the minifilament is a common feature of events with heavy-ion enhancement not ordered by mass. Surprisingly, sources with weak magnetic fields show extreme  $^3\text{He}$  enrichment in these events. Moreover, the energy attained by heavy ions seems to be influenced by the size and form of the jets.

*Unified Astronomy Thesaurus concepts:* Solar energetic particles (1491); Solar abundances (1474); Solar extreme ultraviolet emission (1493); Solar active regions (1974)

*Materials only available in the online version of record: animation*

## 1. Introduction

Owing to their low intensities and the small size of the solar source,  $^3\text{He}$ -rich solar energetic particles (SEPs) are one of the least explored energetic particle populations in the heliosphere. They show enormous enrichment of the rare  $^3\text{He}$  isotope by factors up to  $10^4$  above the coronal or solar wind abundance (G. M. Mason 2007; D. V. Reames 2021a, 2021b). Heavy (Ne–Fe) and ultraheavy ions (mass  $> 70 \text{ AMU}$ ) are enhanced by a factor of 3–10 and  $> 100$ , respectively, independent of the amount of  $^3\text{He}$  enhancement (e.g., G. M. Mason et al. 1986; D. V. Reames et al. 1994; S. T. Hart et al. 2022). The abundance enhancement of heavy ions monotonically increases with ion mass and decreases with charge-to-mass ratio  $Q/M$  (G. M. Mason et al. 2004; D. V. Reames & C. K. Ng 2004).

Solar sources of  $^3\text{He}$ -rich SEPs have been associated with extreme-ultraviolet (EUV) jets (e.g., R. Bučík 2020, and references therein), indicating acceleration at magnetic reconnection sites involving field lines open to interplanetary space (D. V. Reames 2002; Y. M. Wang et al. 2006). It has been suggested that anomalous abundances of  $^3\text{He}$ -rich SEPs are the signature of unique acceleration or heating mechanisms. Most models involve resonant interaction with plasma waves (e.g., L. A. Fisk 1978; M. Temerin & I. Roth 1992; I. Roth & M. Temerin 1997; S. Liu et al. 2004, 2006; Y. Y. Kartavykh

et al. 2020). Other mechanisms encompass ion pickup in the reconnection exhaust (J. F. Drake et al. 2009), Coulomb energy losses (G. M. Mason & B. Klecker 2018), or the first ionization potential (FIP) process (J. M. Laming & N. Kuroda 2023).

In this paper, we investigate the 2023 October 24  $^3\text{He}$ -rich SEP event observed by Solar Orbiter at 0.47 au, showing an extremely high  $^3\text{He}$  abundance with an unusual pattern of heavy-ion elemental composition and species with mass  $\geq 4 \text{ AMU}$  measured only at low energies ( $< 0.5 \text{ MeV nucleon}^{-1}$ ). We include similar, previously reported events (G. M. Mason et al. 2002, 2016, 2023; R. Bučík et al. 2023) and discuss the properties of solar sources given the observed enrichment anomalies. With a novel approach, we estimate the heavy-ion abundance pattern in the 2023 October 24 event using the emission measure (EM) temperature distribution at the solar source for models by L. A. Fisk (1978) and I. Roth & M. Temerin (1997).

## 2. Observations—2023 October 24 Event

### 2.1. Instruments

The elemental composition of the 2023 October 24 event was obtained by the Suprathermal Ion Spectrograph (SIS) of the Energetic Particle Detector (EPD) suite (J. Rodríguez-Pacheco et al. 2020) aboard Solar Orbiter (D. Müller et al. 2020). SIS is a time-of-flight mass spectrometer that measures elemental composition from H through ultraheavy nuclei in the energy range  $0.1\text{--}10 \text{ MeV nucleon}^{-1}$ . SIS has two telescopes, one (SIS-a) pointing at  $30^\circ$  (sunward) and the other (SIS-b) at  $160^\circ$

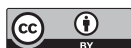

Original content from this work may be used under the terms of the [Creative Commons Attribution 4.0 licence](https://creativecommons.org/licenses/by/4.0/). Any further distribution of this work must maintain attribution to the author(s) and the title of the work, journal citation and DOI.

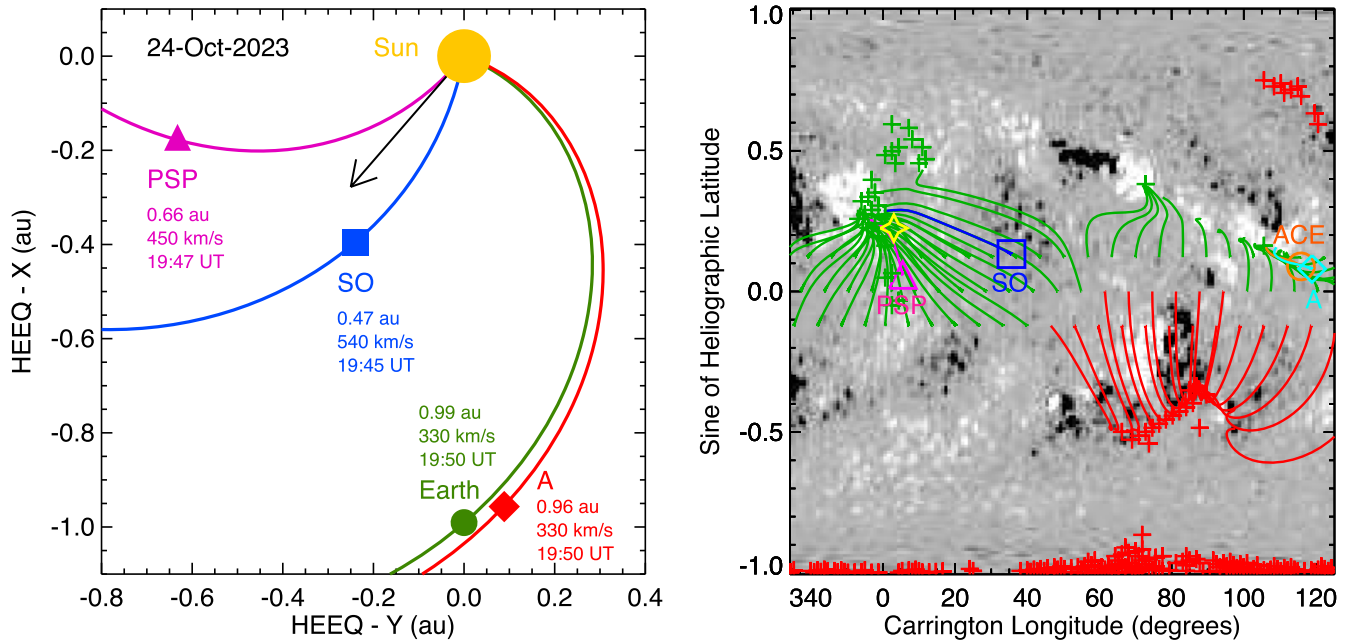

**Figure 1.** Left: location of PSP, Solar Orbiter (SO), Earth, and STEREO-A (A) in Heliocentric Earth Equatorial (HEEQ) coordinates at the time of the event-associated type III radio burst onset observed on each spacecraft. The arrow indicates the SEP source flare. The Parker IMF lines were derived from measured 1 hr averaged solar wind speeds at type III radio burst onset. For PSP, where solar wind speed is not available, we averaged values measured  $\sim 1.5$  days before and  $\sim 2$  days after the type III burst. Heliocentric distance in au and solar wind speed in kilometers per second for respective spacecraft/locations are indicated. Right: photospheric magnetic field map (grayscale), scaled to  $\pm 30$  G for contrast enhancement, and PFSS model of an open coronal field (red is negative and green is positive magnetic polarity). Shown are field lines that intersect the source surface at latitudes  $0^\circ$  and  $\pm 7^\circ$ . Upward triangle, square, circle, and diamond mark the PSP, Solar Orbiter, near-Earth Advanced Composition Explorer (ACE), and STEREO-A magnetic footpoints at the source surface (set at  $2.5 R_\odot$  from Sun center), respectively. The star marks the SEP source flare.

(antisunward) to the west of the spacecraft–Sun line. We also make use of solar wind plasma and interplanetary magnetic field (IMF) measurements from Solar Wind Plasma Analyzer (SWA; C. J. Owen et al. 2020) and the magnetometer (MAG; T. S. Horbury et al. 2020) on Solar Orbiter, respectively. The solar source characteristics of the SEPs were explored using the near-Earth Solar Dynamics Observatory (SDO) with  $0.6 \text{ arcsec pixel}^{-1}$  and 12 s cadence Atmospheric Imaging Assembly (AIA; J. R. Lemen et al. 2012) and  $0.5 \text{ arcsec pixel}^{-1}$  and 45 s and 720 s Helioseismic and Magnetic Imager (HMI; P. H. Scherrer et al. 2012) high-resolution observations. The Solar Orbiter Extreme-Ultraviolet Imager (P. Rochus et al. 2020) high-resolution  $174 \text{ \AA}$  EUV observations (HRI\_EUV\_174;  $0.5 \text{ arcsec pixel}^{-1}$  and 5 s) are not available for the examined event. The Full Sun Imager instrument on Solar Orbiter provided the EUV images at  $174 \text{ \AA}$  and  $304 \text{ \AA}$  with a time resolution of 10 minutes and spatial resolution of  $4.5 \text{ arcsec pixel}^{-1}$ . We examined radio spectrograms for event-associated nonthermal type III radio bursts from the following instruments: Solar Orbiter Radio and Plasma Waves (M. Maksimovic et al. 2020), Parker Solar Probe (PSP) FIELDS (S. D. Bale et al. 2016), Wind WAVES (J. L. Bougeret et al. 1995) and STEREO-A WAVES (J. L. Bougeret et al. 2008).

## 2.2. Magnetic Connection

Figure 1 (left) shows the X–Y plane projection of selected spacecraft in Heliocentric Earth Equatorial (HEEQ) coordinates at the 2023 October 24 event-associated type III radio burst onset. Solar Orbiter observed a type III burst at 19:45 UT, PSP at 19:47 UT, and near-Earth Wind and STEREO-A at 19:50 UT. The type III burst was first visible at approximately 3 MHz at all four spacecraft. Figure 1 (right) displays a photospheric map along with a potential-field source surface

(PFSS) coronal field model on 2023 October 24 at 18:03:28 UT, determined using the SolarSoft (S. L. Freeland & B. N. Handy 1998) `pfss` package.<sup>6</sup> In the package the model is sampled every 6 hr. The photospheric map is generated from HMI magnetograms assimilated into the flux-dispersal model to provide the magnetic field on the full solar sphere (C. J. Schrijver & M. L. De Rosa 2003). Figure 1 (right) shows that PSP and Solar Orbiter are connected to the coronal hole (CH), via open (positive polarity) coronal field lines, where a nearby  $^3\text{He}$ -rich SEP source flare is located. We note that the IMF azimuthal angles on Solar Orbiter were between  $270^\circ$  and  $360^\circ$  (not shown), indicating away or positive polarity, i.e., consistent with the PFSS model. Section 2.4 discusses the identification of the solar source. Unfortunately, the PSP energetic particle instrument IS $\odot$ IS (M. E. Hill et al. 2017) experienced a data gap on October 25 from 04:00 to 23:00 UT, when Solar Orbiter observed a substantial part of the event.

## 2.3. Energetic Particles

Figure 2 plots the elemental composition measurements and context solar wind data from Solar Orbiter for the 2023 October 24  $^3\text{He}$ -rich event. Enhanced total pressure during the gradual solar wind speed increase (from  $\sim 300$  to  $\sim 600 \text{ km s}^{-1}$  in 1.5 days), a typical characteristic of corotating interaction regions (CIRs; L. F. Burlaga 1995), is seen in Figure 2(a) (marked by dotted magenta lines). Furthermore, the gradual change in flow direction from west to east, another CIR characteristic, started at 19:30 UT on October 23, around the beginning of the solar wind speed increase (not shown). The

<sup>6</sup> <https://www.lmsal.com/~derosa/pfsspack/>

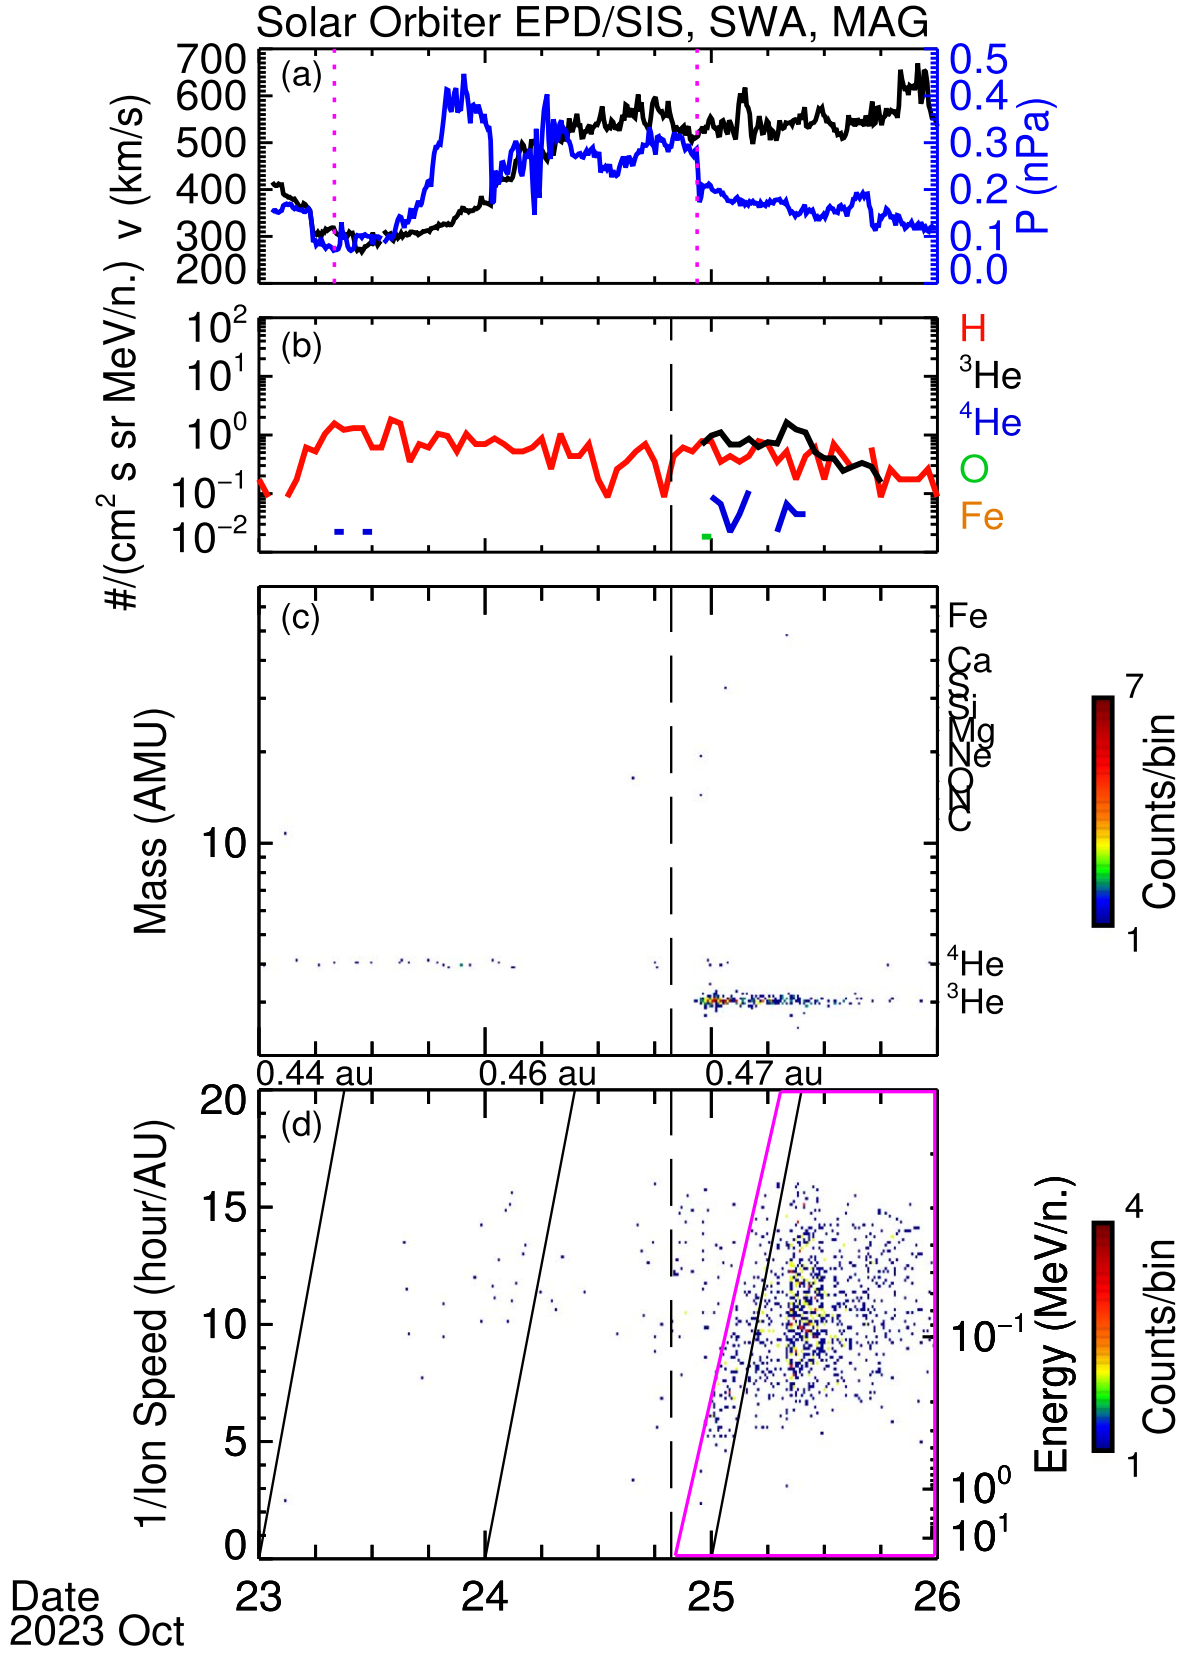

**Figure 2.** Solar Orbiter measurements. (a) 10 minutes solar wind speed (black) and total pressure (blue). A pair of vertical magenta dotted lines approximately marks CIR. (b) 1 hr ion intensities at 0.23–0.32 MeV nucleon<sup>-1</sup>. (c) Mass vs. time at 0.4–10 MeV nucleon<sup>-1</sup>. (d) 1/ion speed vs. arrival times of 10–70 AMU ions. Slanted lines mark arrival times for particles traveling along the nominal Parker field line without scattering. The trapezoid, highlighted in magenta, marks the period where the energy spectra and elemental ratios were calculated. Heliocentric distances in au at the beginning of each day are displayed. The measurements in panel (b) are from both SIS telescopes and panels (c)–(d) from SIS-a. The vertical black dashed line indicates the onset of the type III radio burst at Solar Orbiter (19:45 UT).

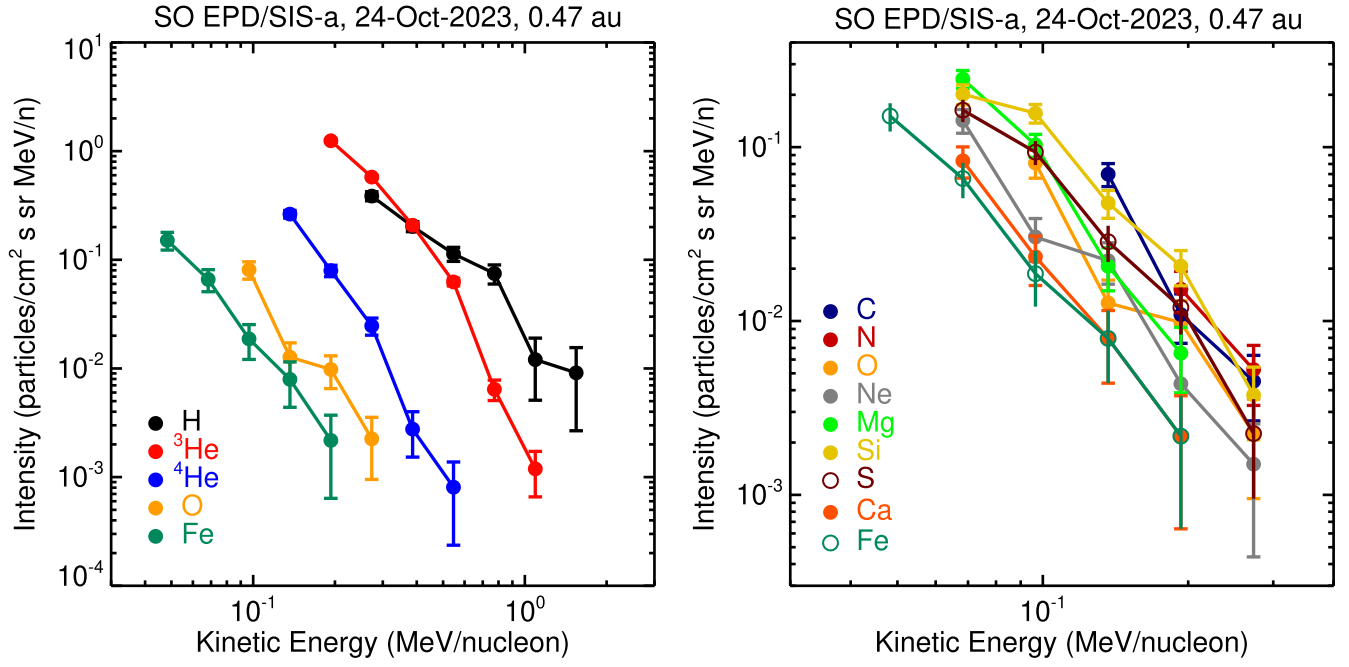

Figure 3. Intensity spectra for selected ion species measured by SIS-a at the 2023 October 24 event.

total pressure  $P$  is given by the sum of the plasma and magnetic field pressure, i.e.,  $P = 2n_p k T_p + B^2/2\mu_0$ , where  $n_p$  and  $T_p$  are the proton density and temperature, respectively, and  $B$  is the magnetic field magnitude. In Figure 2(b), the H intensity does not show any rise in coincidence with the  $^3\text{He}$ , although the  $^4\text{He}$  does. So, the H is not due to the  $^3\text{He}$  injection. The panel shows that the H intensity increase started at  $\sim 03:00$  UT on October 23 in association with the CIR and may dominate the  $^3\text{He}$ -rich SEP event during October 24–25. CIR ion intensity enhancements typically extend beyond CIR trailing edges and may last several days (e.g., R. Bučík et al. 2009; R. W. Ebert et al. 2012). Remarkably, the mass versus time spectrogram at energy  $0.4\text{--}10\text{ MeV nucleon}^{-1}$  in Figure 2(c) shows almost exclusively  $^3\text{He}$ , with only a few other ion species measured above an energy of  $\sim 0.4\text{ MeV nucleon}^{-1}$ . The velocity dispersion pattern on October 24 in Figure 2(d) suggests the ion solar release time coincided with a type III burst at 19:45 UT. The onset of the event at PSP was not measured. Either the onset moved to the data gap because of the particle’s later arrival at PSP (e.g., 1 hr for  $0.4\text{ MeV nucleon}^{-1}$ ), or the event was too small to be measured at further distances from the Sun.

Figure 3 shows intensity energy spectra for various ion species for the 2023 October 24 event. We focus on heavy ions, as H is likely dominated by the CIR event. The heavy-ion spectra are similar to each other, with a power-law-like shape. The  $^3\text{He}$  spectrum faintly bends toward low energies below  $\sim 0.5\text{ MeV nucleon}^{-1}$ , bringing the  $^3\text{He}/^4\text{He}$  ratio to increase with energy. Figure 3 (left) shows that  $^3\text{He}$  (except H, which is most likely all CIR) significantly dominates all species, and O prevails over Fe. The  $^3\text{He}$  looks similar to Fe and is shifted to higher energy by a factor of  $\sim 7$ , larger than the average shift factor of  $3 \pm 1.3$  in G. M. Mason et al. (2024). An unusual feature seen in Figure 3 (right) is the dominance of lighter species (C, N, Ne, Mg, Si, S) over Fe. Interestingly, while  $^3\text{He}$  extends to  $\sim 1\text{ MeV nucleon}^{-1}$ , heavy ions (C–Fe) show spectral points below  $\sim 0.2\text{--}0.3\text{ MeV nucleon}^{-1}$ . Because C and N are

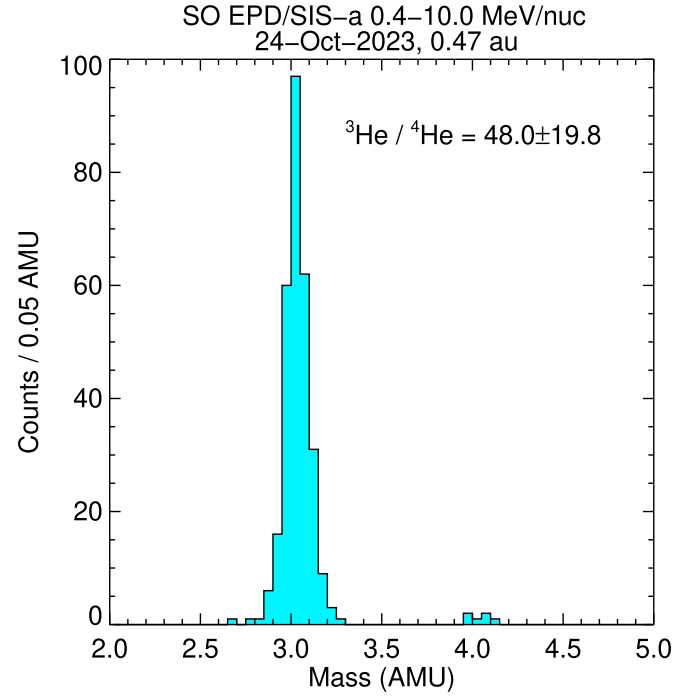

Figure 4. SIS-a He mass histogram for the 2023 October 24 event in the energy range  $0.4\text{--}10.0\text{ MeV nucleon}^{-1}$ .

not well resolved at low energies, their low-energy spectral points are not displayed.

Figure 4 shows the SIS-a He histogram for the examined event at  $0.4\text{--}10.0\text{ MeV nucleon}^{-1}$  in the trapezoid range shown in magenta color in Figure 2(d). The  $^3\text{He}/^4\text{He}$  ratio is  $48.0 \pm 19.8$  at  $0.4\text{--}10.0\text{ MeV nucleon}^{-1}$ , with a relatively high error (41%) owing to the small number (six) of  $^4\text{He}$  counts. Note that in the same energy range and integration period, only four ions at  $10\text{--}70\text{ AMU}$  were detected (see Figure 2(c)). The ratio remains unchanged after decreasing the upper energy value to  $3.0\text{ MeV nucleon}^{-1}$ . The  $^3\text{He}/^4\text{He}$  ratio at  $0.1600\text{--}0.2263$ ,



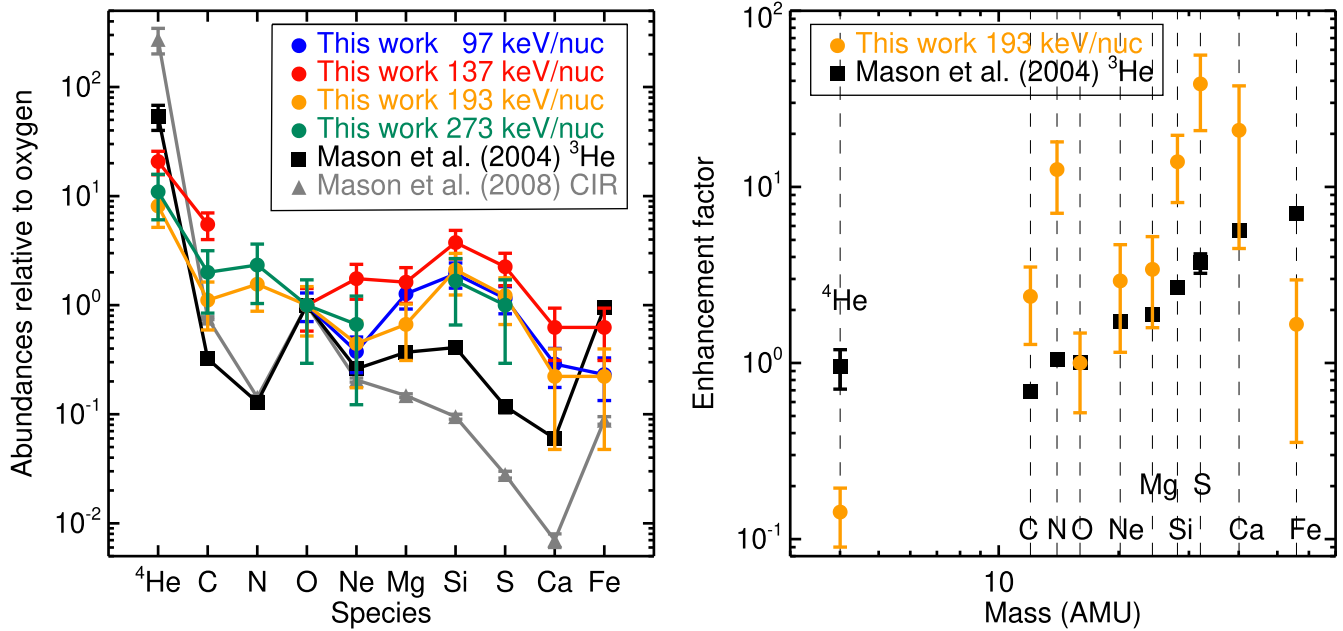

**Figure 5.** Left: SIS-a 0.097, 0.137, 0.193, and 0.273 MeV nucleon $^{-1}$  abundances relative to O for the 2023 October 24 event (circles). Overplotted are 0.386 MeV nucleon $^{-1}$  ion abundances from the  $^3\text{He}$ -rich SEP event survey by G. M. Mason et al. (2004) and the CIR event survey by G. M. Mason et al. (2008). Right: abundance enhancement factor relative to O for the 2023 October 24 event (at 0.193 MeV nucleon $^{-1}$ ) relative to coronal abundances from D. V. Reames (1995). Black squares are values from the G. M. Mason et al. (2004)  $^3\text{He}$ -rich SEP survey at 0.386 MeV nucleon $^{-1}$ .

0.2263–0.3200, and 0.3200–0.4525 MeV nucleon $^{-1}$  is  $15.67 \pm 1.95$ ,  $23.39 \pm 4.29$ , and  $75.20 \pm 33.85$ , respectively. The latter extremely high ratio is  $\sim 1.8 \times 10^5$  times the slow solar wind value of  $(4.08 \pm 0.25) \times 10^{-4}$  (R. Bodmer et al. 1995; G. Gloeckler & J. Geiss 1998).

Figure 5 (left) displays relative abundances for the 2023 October 24 event and  $^3\text{He}$ -rich SEP (G. M. Mason et al. 2004) and CIR (G. M. Mason et al. 2008) reference elemental composition. In the examined event, the abundances at 0.137 MeV nucleon $^{-1}$  are systematically higher by a factor of  $\sim 2$ – $3$  compared to the abundances at 0.097, 0.193, and 0.273 MeV nucleon $^{-1}$  (when available) for all species except for C and Ne, whose 0.137 MeV nucleon $^{-1}$  abundances are a factor of  $\sim 4$ – $5$  higher. The abundances at 0.097, 0.193, and 0.273 MeV nucleon $^{-1}$  for  $^4\text{He}$ , Si, S, Ca, and Fe differ within a factor of 1 between these three energies and for C, N, Ne, and Mg within a factor of 2. The abundances of  $^4\text{He}$  and Fe are lower than the reference values reported by G. M. Mason et al. (2004). The abundances of all other species show higher values than the  $^3\text{He}$ -rich SEP reference composition, although 0.193 MeV nucleon $^{-1}$  Ca, Mg, and Ne, and 0.273 MeV nucleon $^{-1}$  Ne are within statistical uncertainties. Although the error is large, the elevated C/O ratio is puzzling. It is more characteristic of CIR or solar wind abundances (D. V. Reames et al. 1991; G. M. Mason et al. 2008). Two species,  $^4\text{He}$  and C, have higher abundances in CIR events than in  $^3\text{He}$ -rich SEP events. Since the  $^4\text{He}$  abundance in the event is smaller than typical  $^3\text{He}$ -rich SEP abundances, it is unlikely that the CIR contributes just to the C abundance enhancement.

Figure 5 (right) plots the abundance enhancement factor  $(X/O)/(X/O)_{\text{corona}}$  of element X for the investigated  $^3\text{He}$ -rich SEP event at 0.193 MeV nucleon $^{-1}$  (where abundances for all species are available) versus mass. The coronal abundances are represented by 5–12 MeV nucleon $^{-1}$  gradual SEP abundances taken from D. V. Reames (1995). All abundances are normalized to O. Shown are the average values from the G. M. Mason et al. (2004) survey of 20  $^3\text{He}$ -rich SEP events,

where enhancements are also against gradual SEP abundances from D. V. Reames (1995). The enhancement pattern in the 2023 October 24 event is irregular. It does not show a smooth rise with mass. In addition, the enhancement factor through Mg–Si–S increases steeply with mass, in a factor of 10+, compared to a factor of 2 in a typical  $^3\text{He}$ -rich SEP event. A notable feature is the large enhancement of N, Si, and S and a decline in Fe and  $^4\text{He}$ . Table 1 gives the abundances and enhancement factors for the examined event and G. M. Mason et al. (2004) survey, shown in Figure 5. The abundances of the best-observed event (2014 May 16) from the G. M. Mason et al. (2016) survey of  $^3\text{He}$ -rich SEP events with atypical enhancement patterns are listed.

#### 2.4. Solar Source

Figure 6 displays the solar source of the investigated event in the AIA 211 Å image and 45 s HMI line-of-sight (LOS) magnetogram at the time of the event-associated type III radio burst (as observed at 1 au where the images were obtained). The solar source (a bright point), marked by arrows in Figures 6(a)–(b), is located near the edge of the low-latitude CH (dark area in the AIA 211 Å direct image). The CH boundary, highlighted in red contours, was obtained from the SolarSoft Collection of Analysis Tools for Coronal Holes (S. G. Heinemann et al. 2019). Stonyhurst’s heliographic longitude and latitude of the solar source are  $-43^\circ$  (E43) and  $13^\circ$  (N13), respectively. Note that the Carrington longitude of the source is  $3^\circ$  (see Figure 1, right panel). The solar source was identified using a standard approach based on the temporal coincidence between EUV brightening observed on the solar disk and the event-associated type III radio burst. Figures 6(a)–(b) show that the only brightening was one near the CH (see also the animation segment corresponding to Figure 6(b)). The animation segment relating to Figure 6(c) reveals an eruption of the dark (cool) minifilament of an S-like shape at around 19:48 UT. Simultaneously, the brightness at the source notably

**Table 1**  
Abundances and Enhancement Factors

| Element         | Abundances         |                    |                    |                    | Enhancement Factors                              |                    |                                   |                    |
|-----------------|--------------------|--------------------|--------------------|--------------------|--------------------------------------------------|--------------------|-----------------------------------|--------------------|
|                 | 2023 Oct 24        |                    |                    |                    | G. M. Mason et al. (2004)                        |                    | G. M. Mason et al. (2004)         |                    |
|                 | 0.097 <sup>b</sup> | 0.137 <sup>b</sup> | 0.193 <sup>b</sup> | 0.273 <sup>b</sup> | 2014 May 16 <sup>a</sup><br>0.4–1.0 <sup>b</sup> | 0.386 <sup>b</sup> | 2023 Oct 24<br>0.193 <sup>b</sup> | 0.386 <sup>b</sup> |
| <sup>4</sup> He | ...                | 20.7 ± 5.0         | 8.12 ± 2.95        | 11.0 ± 4.9         | 79.53 ± 9.70                                     | 54 ± 14            | 0.14 ± 0.05                       | 0.95 ± 0.24        |
| C               | ...                | 5.50 ± 1.51        | 1.11 ± 0.52        | 2.00 ± 1.15        | 1.13 ± 0.17                                      | 0.322 ± 0.003      | 2.40 ± 1.16                       | 0.69 ± 0.01        |
| N               | ...                | ...                | 1.56 ± 0.68        | 2.33 ± 1.30        | 0.97 ± 0.15                                      | 0.129 ± 0.002      | 12.5 ± 5.5                        | 1.04 ± 0.03        |
| O               | ≡ 1.0 ± 0.29       | ≡ 1.0 ± 0.42       | ≡ 1.0 ± 0.48       | ≡ 1.0 ± 0.71       | ≡ 1.0 ± 0.15                                     | ≡ 1.0 ± 0.006      | ≡ 1.0 ± 0.48                      | ≡ 1.0 ± 0.01       |
| Ne              | 0.38 ± 0.14        | 1.75 ± 0.62        | 0.44 ± 0.27        | 0.67 ± 0.54        | 0.58 ± 0.10                                      | 0.261 ± 0.003      | 2.92 ± 1.77                       | 1.72 ± 0.05        |
| Mg              | 1.27 ± 0.35        | 1.63 ± 0.58        | 0.67 ± 0.36        | ...                | 0.61 ± 0.11                                      | 0.370 ± 0.003      | 3.40 ± 1.81                       | 1.89 ± 0.04        |
| Si              | 1.93 ± 0.50        | 3.75 ± 1.10        | 2.11 ± 0.87        | 1.67 ± 1.00        | 3.68 ± 0.45                                      | 0.409 ± 0.004      | 13.9 ± 5.7                        | 2.69 ± 0.07        |
| S               | 1.15 ± 0.32        | 2.25 ± 0.74        | 1.22 ± 0.56        | 1.00 ± 0.71        | 3.83 ± 0.46                                      | 0.118 ± 0.015      | 38.4 ± 17.6                       | 3.70 ± 0.47        |
| Ca              | 0.29 ± 0.11        | 0.63 ± 0.31        | 0.22 ± 0.17        | ...                | 0.45 ± 0.18                                      | 0.060 ± 0.003      | 21.0 ± 16.5                       | 5.66 ± 0.38        |
| Fe              | 0.23 ± 0.10        | 0.63 ± 0.31        | 0.22 ± 0.17        | ...                | 3.00 ± 0.37                                      | 0.950 ± 0.005      | 1.66 ± 1.30                       | 7.09 ± 0.21        |

**Notes.**

<sup>a</sup> Event in G. M. Mason et al. (2016).

<sup>b</sup> MeV nucleon<sup>-1</sup>.

increases. This is followed by a jet ejection observed at around 19:53 UT in the southeast direction. Except for 211 Å, the minifilament was observed in the 193, 171, 131, and 304 Å wavelengths. The yellow rectangle enclosing the solar source (and base of the jet) has a diagonal of 34 Mm, the size of a supergranulation scale ( $\sim 30$  Mm; M. Rieutord & F. Rincon 2010). The bright area, a plage, eastward from  $-50^\circ$ , corresponds to relatively high concentrations of strong positive (white) polarity magnetic fields in the LOS magnetogram (see Figures 6(c)–(d)). The remaining area on the west contains weak (gray) magnetic fields of the CH with several magnetic elements, mostly of positive polarity. The unsigned (total) mean magnetic field strength in the rectangle surrounding the source is  $\sim 8$  G, significantly lower than fields in active regions (ARs). It was obtained by averaging absolute values of the magnetic field strength of each pixel (there were 4000 pixels in the rectangle). We use the 720 s magnetogram at 19:58 UT (the closest one to the type III radio burst) due to lower photon noise than the 45 s magnetogram. After correction for angular distance from the center of the solar disk, the value is  $\sim 11$  G. Figure 7(a) shows a minifilament in the source of the October 24 event about 1 minute before its eruption, and Figure 7(b) shows a weak straight jet that has a size similar to its base. Previous studies have reported the eruption of a minifilament as a trigger of coronal jets (e.g., A. C. Sterling et al. 2016; N. K. Panesar et al. 2016).

No GOES X-ray flare was observed in association with this event. We note that the C1.3 GOES X-ray flare at 19:53 UT and a maximum at 20:18 UT occurred on the east limb (S13E88). The solar source of the investigated event was coincidentally captured by the Interface Region Imaging Spectrograph (B. De Pontieu et al. 2014) observatory in its limited field of view ( $165 \times 175$  arcsec<sup>2</sup>) in Si IV 1400 Å and Mg II k 2796 Å slit-jaw UV images. However, spectra cannot be obtained around the time of the type III radio bursts since the slit passed through the source at 20:13 UT, i.e., when the eruption had already ceased.

### 2.5. Solar Source Temperature

Differential emission measure (DEM) was previously used to determine the temperature at the solar source in 24 <sup>3</sup>He-rich SEPs events (R. Bučík et al. 2021). The authors calculated the

EM-weighted temperature at the time of the event-associated type III radio burst. This method provided a reasonable agreement with temperature obtained from in situ Fe charge states at  $\sim 0.1$  MeV nucleon<sup>-1</sup> (R. DiFabio et al. 2008) and the elemental abundance measurements (e.g., D. V. Reames et al. 2014). Here, we use EM to derive the temperature and its evolution at the solar source of the 2023 October 24 event. DEM is a physical quantity related to the electron number density and temperature gradient of a plasma. It is determined from observations of emission lines on the assumption that plasma is optically thin and in ionization equilibrium. The DEM is reconstructed from multiwavelength observations and the instrumental temperature response by the inversion method. We use the DEM inversion developed by M. C. M. Cheung et al. (2015) for EUV AIA imaging observations.<sup>7</sup> We coalign AIA images in six channels (94, 131, 171, 193, 211, and 335 Å), which are sensitive to a range of temperatures (B. O'Dwyer et al. 2010; G. Del Zanna et al. 2011; G. Del Zanna 2013), and use them as input in the EM analysis. We computed the AIA temperature response function using the technique given by G. Del Zanna et al. (2011). We created an isothermal spectrum using the latest CHIANTI version (K. P. Dere et al. 2019), the electron number density of  $1 \times 10^{10}$  cm<sup>-3</sup>, and coronal abundances (Sun\_coronal\_2021\_chianti.abund; available in the CHIANTI database). This spectrum was then folded with the effective area of each AIA filter (obtained using the SolarSoft routine `aia_get_response.pro`), and temperature responses were obtained. The EM (the integral of the DEM) is computed for each pixel position in the solar source and its surrounding area, and the temperature interval  $\log T$  (K) = 5.4–7.5 (0.3–30 MK). Finally, the EM is spatially averaged over the rectangular region around the source (shown as a white box in Figure 8). The region was selected to contain EUV brightening in running difference images at type III radio burst onset (R. Bučík et al. 2021). The DEM inversion code gives temperature within an error of 20%. The errors arise from instrumental effects and photon counting statistics.

Figure 8 shows EM maps at various temperature intervals at the solar source and its surroundings for the 2023 October 24

<sup>7</sup> [https://www.lmsal.com/~cheung/AIA/tutorial\\_dem/](https://www.lmsal.com/~cheung/AIA/tutorial_dem/)



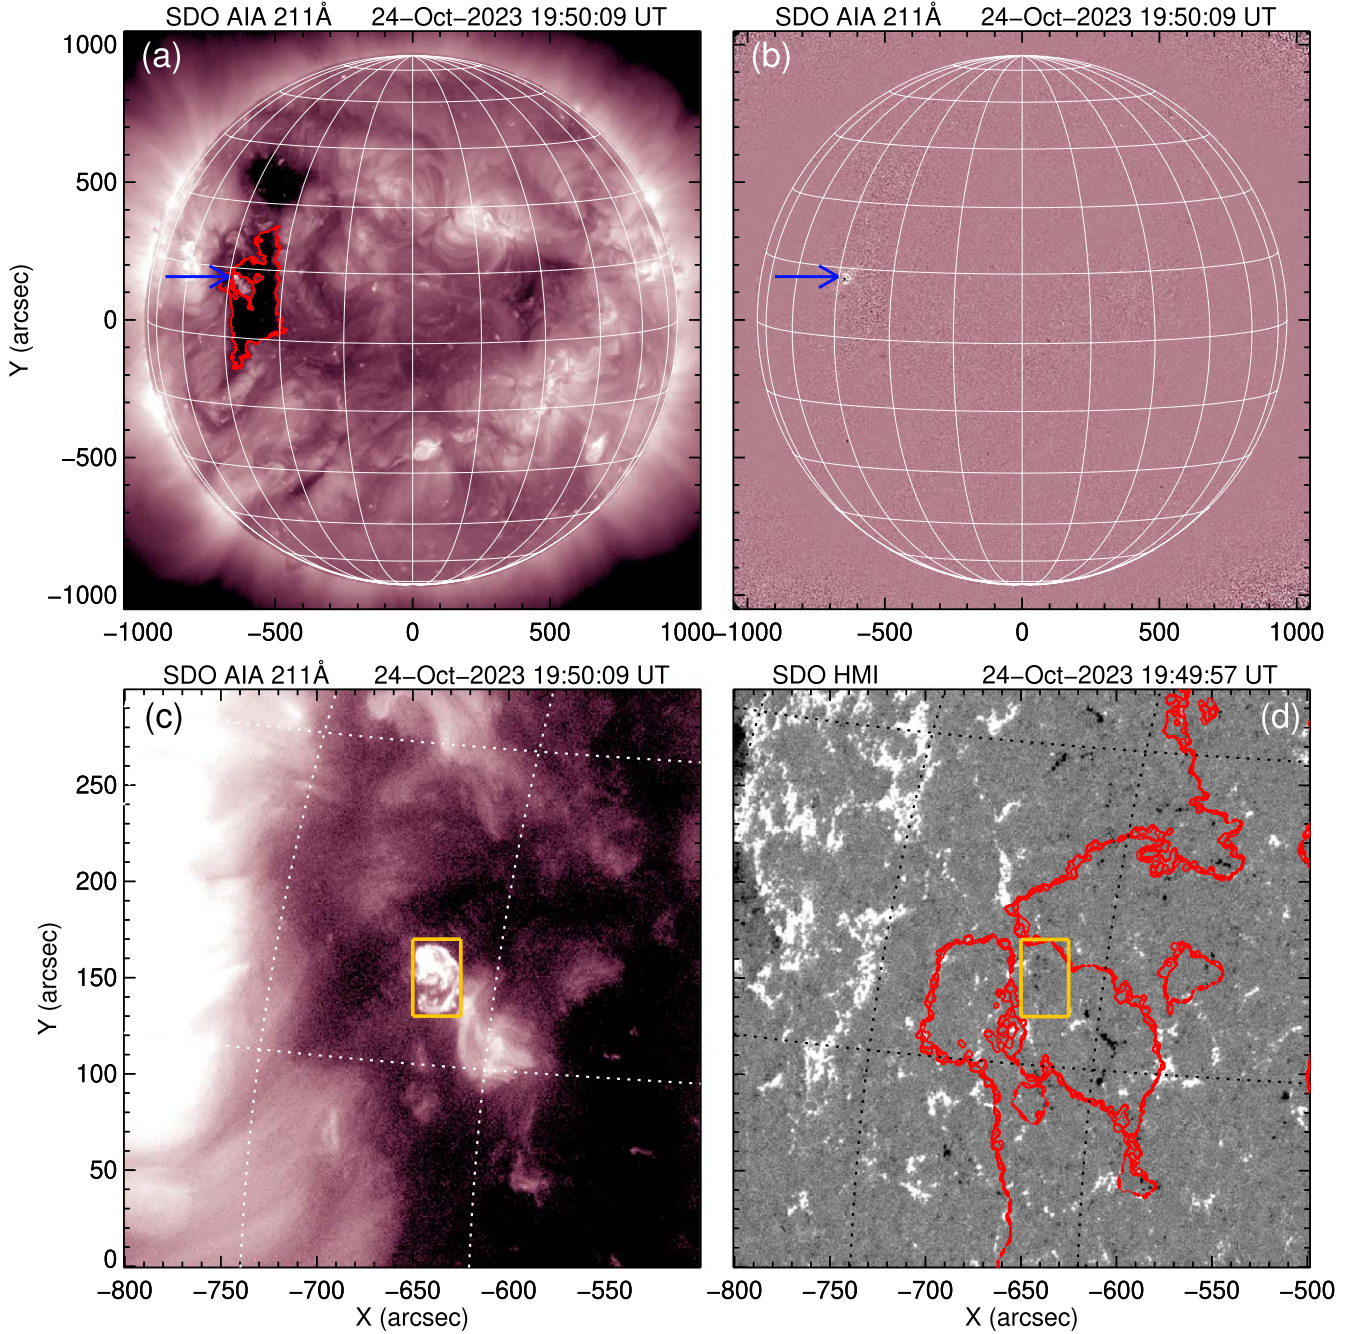

**Figure 6.** (a) Direct and (b) 1 minute running difference SDO/AIA EUV 211 Å images of the solar disk. Arrows point to the solar source of the  $^3\text{He}$ -rich SEPs in the 2023 October 24 event. The red contour marks a coronal hole (CH) near the solar source. (c) Zoom-in view of the area around the solar source in the direct AIA EUV 211 Å image and (d) the SDO 45 s HMI LOS magnetogram scaled to  $\pm 100$  G. The red contour of the CH is overplotted. The yellow rectangles enclose the solar source. Images are at the time of the event-associated type III radio burst onset. The Stonyhurst grid has  $15^\circ$  ( $10^\circ$ ) spacing in the (a)–(b) ((c)–(d)) panels. An animation at 19:45:09–19:58:09 UT corresponding to panel (b) and 19:44:57–19:59:45 UT corresponding to panel (c) is available. The real-time duration of the animation is 4 s. The first second shows the panel (b) sequence with the remaining time for panel (c).

(An animation of this figure is available in the [online article](#).)

$^3\text{He}$ -rich SEP event at the time of the event-associated type III radio burst. The solar source is bounded by a white rectangle, the same as in Figures 6(c) and (d). We obtained such maps between 19:39 UT and 20:05 UT with a temporal resolution of 12 s.

Figure 9 shows the color-coded EM in a temperature versus time diagram on 2023 October 24 from 19:39 to 20:05 UT. The EM is spatially averaged in the area bounded by the rectangle in Figure 8. Between 19:39 and 19:47 UT, 1.3 MK ( $\log T$  6.1 K)

and 1.6 MK ( $\log T$  6.2 K) dominate the region as they have the highest and the same EMs. At 19:48 UT (minifilament eruption), the EM starts increasing, but 1.3 and 1.6 MK still dominate. At 19:49 UT, 1.6 and 2.0 MK ( $\log T$  6.3 K) dominate. Between 19:50 UT (type III burst onset) and 19:56 UT, 2.0 MK dominates the source region. Later, lower temperatures again prevail. At 19:50 UT, the region also clearly shows temperatures around 0.3 MK ( $\log T$  5.4 and 5.5 K), though with a factor of 3 lower EMs than 2 MK (see Figure 11(c)).

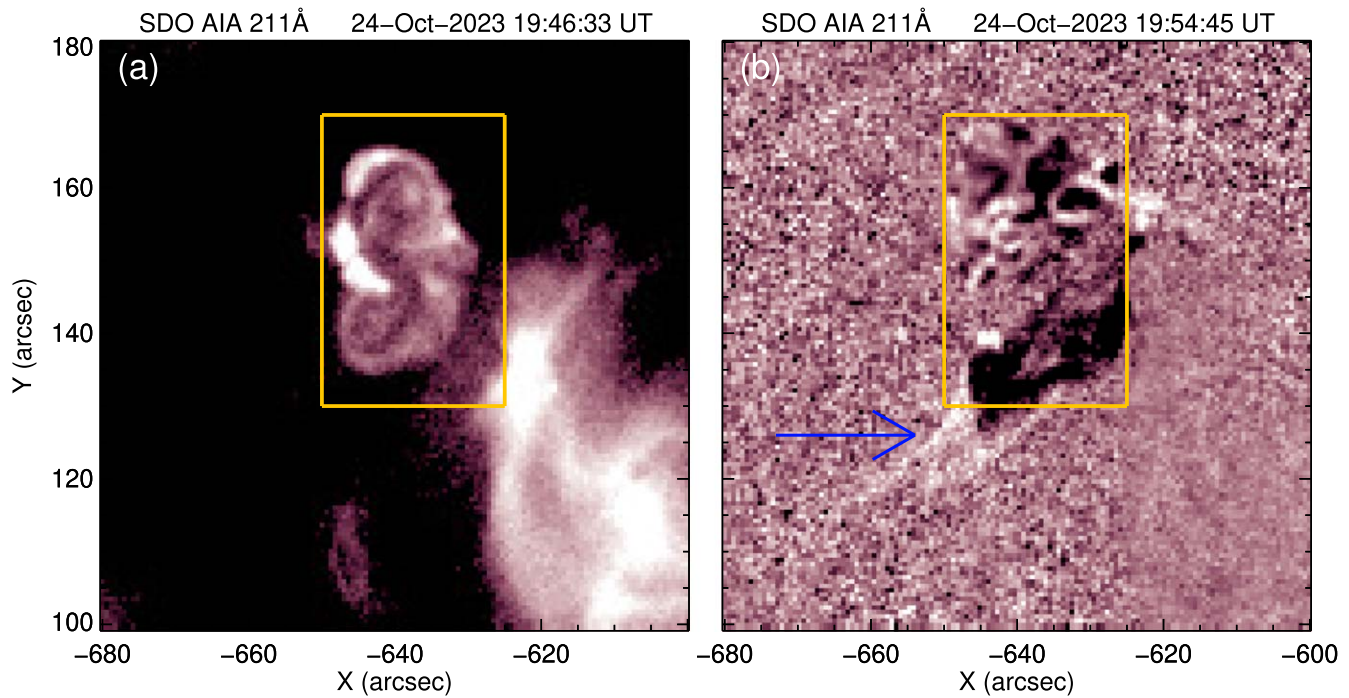

**Figure 7.** (a) Direct AIA EUV 211 Å image of a minifilament (dark S-like shape, whose upper segment is bounded from outside by a brightening) in the solar source. (b) 1 minute running difference AIA EUV 211 Å image of a jet (marked by an arrow) ejected from the solar source. The yellow rectangles enclose the solar source.

### 3. Discussion

#### 3.1. Solar Sources of Previously Reported Similar Events

G. M. Mason et al. (2002, 2016) reported 17 events measured by the Advanced Composition Explorer in 1997–2015 showing no simple heavy-ion enhancement pattern with mass, with greatly enhanced C/O, N/O, Si/O, and S/O over average values in  $^3\text{He}$ -rich SEP events. Two other events were reported from Solar Orbiter observations (R. Bučík et al. 2023; G. M. Mason et al. 2023). For most of these events, spectra were measured below 1 MeV nucleon $^{-1}$ . Table 2 summarizes the sources of these events. Column (1) lists the event number. Column (2) provides the  $^3\text{He}$ -rich SEP event start date. Column (3) indicates with Y (yes) or N (no) the presence of a CH. Columns (4), (5), and (6) give EUV flare type, location, and time, respectively. The EUV refers to the 195 Å Solar and Heliospheric Observatory (SOHO) Extreme-ultraviolet Imaging Telescope (EIT; J. P. Delaboudinière et al. 1995) for #1–2 and #8–9, 193 Å SDO/AIA for #11–14 and #16–18, and 195 Å STEREO-A Extreme Ultraviolet Imager (EUVI; R. A. Howard et al. 2008) for #15. Column (7) indicates the observation of an erupting minifilament in EIT 195 Å (SOHO 304 Å images were not available) or AIA (EUVI) 304 Å. Column (8) provides the start time of type III radio bursts from Wind WAVES (#2, #4–17), STEREO-A WAVES (#18), and the US National Oceanic and Atmospheric Administration (NOAA) Edited Events catalog (#3). Column (9) lists the  $^3\text{He}/^4\text{He}$  ratio at 0.5–2.0 MeV nucleon $^{-1}$  (#1–3, #5–17) and 0.32–0.45 MeV nucleon $^{-1}$  (#18–19). In the 2023 October 24 event, the  $^3\text{He}/^4\text{He}$  at 0.5–2.0 MeV nucleon $^{-1}$  is  $28.5 \pm 14.5$ . The last column provides the EM-weighted temperatures.

Twelve events in Table 2 had previously identified sources. These solar sources are displayed in Figure 10: #1–2, #8–9 in SOHO images, #11–14, #16–18 in SDO, and #15 in STEREO-A images. The solar sources of four events, #1–2 and #8–9, were inspected by Y. M. Wang et al. (2006) with

SOHO EIT (2.6 arcsec pixel $^{-1}$  and 12 minutes) 195 Å images and nearby CHs with near-infrared He I 10830 Å data from the National Solar Observatory Kitt Peak. Y. M. Wang et al. (2006) explored  $^3\text{He}$ -rich SEP events from 1997 to 2003 whose sources the authors were able to identify. Table 2 includes 10 events in this period, but only four of them have been reported by Y. M. Wang et al. (2006). The sources of events #3–7 and #10 were presumably too small to be resolved by EIT. The same applies to minifilament identification in events #1–2 and #8–9, though some hints of narrow dark features, resembling a minifilament, could be observed in sources for events #2 and #8. For event #1, only half-spatial-resolution EIT images are available. The photospheric field underneath the solar sources in events #1–2 and #8–9 is shown in SOHO 2 arcsec pixel $^{-1}$  and 96 minutes cadence Michelson Doppler Imager (MDI; P. H. Scherrer et al. 1995) magnetograms. The minifilaments in events #16 (N. V. Nitta et al. 2015; D. E. Innes et al. 2016; G. M. Mason et al. 2016) and #18 (R. Bučík et al. 2023) were identified in earlier studies. Event #18 in Table 2 (event #5 in R. Bučík et al. 2023) was one of the six recurrent  $^3\text{He}$ -rich SEP events measured on March 3–6 by Solar Orbiter at  $\sim 0.5$  au. Remarkably, the recurrent event with the minifilament eruption was rich in Si–S. Event #19, observed by Solar Orbiter at 0.29 au, had an uncertain solar source. The solar source in event #14 is noticeably different—it is larger and hotter. The arrow in the source for this event points to the faint dark feature (possible minifilament). This is also a site with fast changes in the brightening. The photospheric field underneath the solar sources for events #11–14 and #16–17 is displayed in HMI magnetograms. We note that event #15 with a source behind the limb, observed by STEREO-A, has no magnetogram observations (therefore a blank space in Figure 10). A minifilament in this event was inspected with 304 Å EUVI images (1.6 arcsec pixel $^{-1}$  and 2.5 minutes).



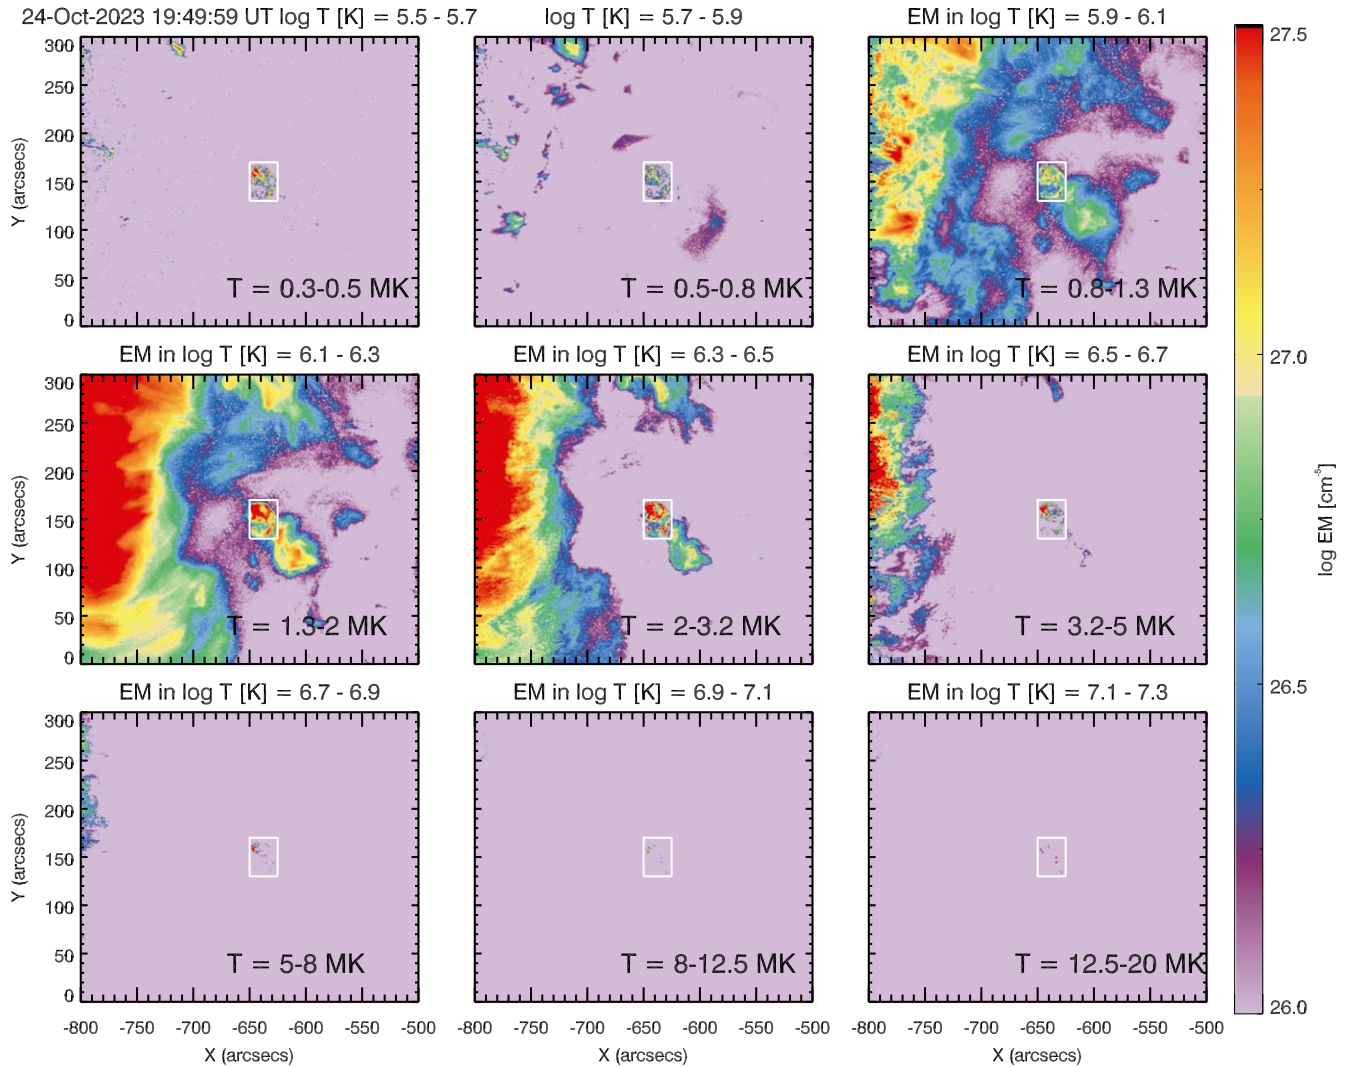

**Figure 8.** Emission measure (EM) maps for the 2023 October 24 event at the start time of the type III radio burst. The white rectangle surrounds the source region, where the temperature was determined. Color-coding indicates the total EM contained within a  $\log T$  range, shown at the top of each panel.

The underlying photospheric field for events in Figure 10 is fairly variable. We observe relatively small magnetic elements, suggesting a weak surface field (class I), in events #1, #2, and #16. The 2023 October event is in this category. Bipolar ARs (class II) are seen in events #8, #9, #11, and #12 (see R. Bučík et al. 2014, for #11). A plage region (class III) was previously reported in event #13 (N.-H. Chen et al. 2015) and #18 (R. Bučík et al. 2023). Finally, large sunspots with magnetic moving features of opposite polarity (class IV) are seen in events #14 and #17. Remarkably, the events with the highest  $^3\text{He}/^4\text{He}$  ratios (#2 and #16) have a class I solar source, while the lowest  $^3\text{He}/^4\text{He}$  (except #11) have class II and IV sources. Note that the AR in event #11 with a rather high  $^3\text{He}/^4\text{He}$  ratio was a newly emerging region within the CH (R. Bučík et al. 2014), characterized by a weak field.

### 3.2. Solar Source of 2023 October 24 Event

G. M. Mason et al. (2002, 2016) suggested that cool material must be present at the source, producing ionization states for selective C, N, Si, and S enhancement, and not allowing temperatures high enough to bring Ca and Fe to the required ionization states. G. M. Mason et al. (2016) discussed the cool

minifilament observed in event #16. Remarkably, a minifilament was observed not only in the 2023 October event but virtually in all other sources in Table 2 when resolution allowed identification. Furthermore, it has been suggested that such enhancement is produced by a range of temperatures occurring subsequently as the plasma is heated from initial low temperatures (e.g., G. M. Mason et al. 1980, 2016). Specifically, a large enhancement of N and Si could be produced by resonant heating with the same waves of ionization states of these ions that occur at different temperatures (G. M. Mason et al. 2002). Furthermore, G. M. Mason et al. (1980) suggested that waves need to be generated repeatedly during the heating phase. Here, we show that various temperatures may coexist at a source of  $^3\text{He}$ -rich SEPs (Figure 9). This may suggest that common enhancement of lighter and heavier ion species would not necessarily need to be achieved subsequently but could happen in a single episode (or finite short time), e.g., during a stage when magnetic reconnection produces the required waves. D. V. Reames (2023) argued that reconnection and particle acceleration occur rapidly, early, before much heating.

The 2023 October 24 event shows extremely large  $^3\text{He}$  enrichment. Event #2 has the greatest  $^3\text{He}/^4\text{He}$  ratio in Table 2 ( $33.4 \pm 5.2$  at  $0.385 \text{ MeV nucleon}^{-1}$ ; G. M. Mason et al. 2000),

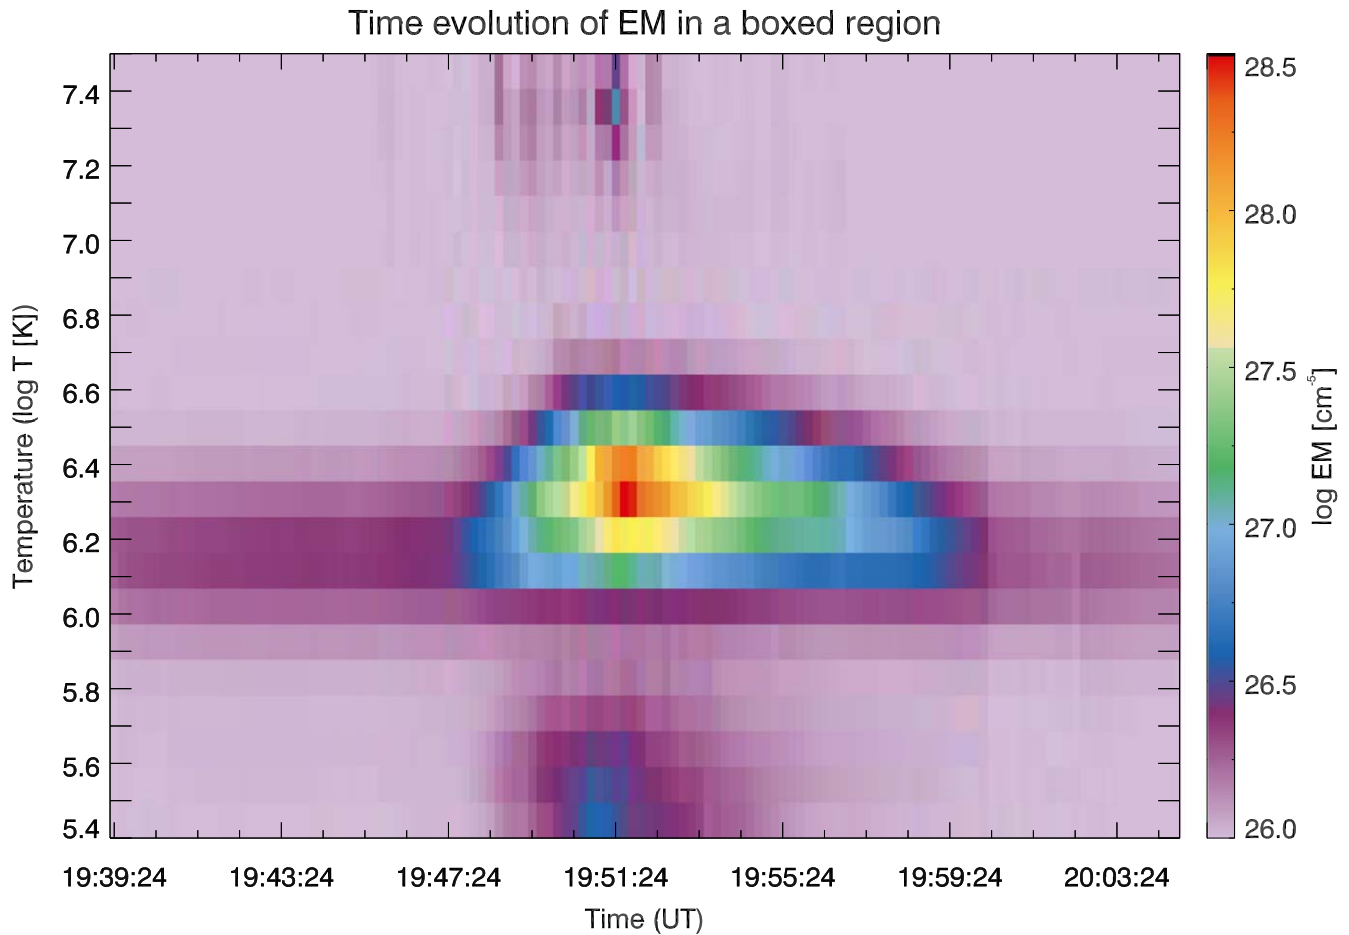

**Figure 9.** Temperature vs. time in the rectangle around the SEP source. The spatially averaged emission measure (EM) is color-coded.

and event #16 has the second-highest  ${}^3\text{He}$  enrichment. A common feature of these three events is their surface magnetic field (class I). S. Liu et al. (2006) pointed out that situations with weak turbulence produce higher  ${}^3\text{He}$  enrichments than cases with strong turbulence (see also Figure 8 in G. M. Mason et al. 2024). The authors also concluded that in a strongly magnetized plasma, the  ${}^3\text{He}$  enhancement decreases. These model outcomes are qualitatively consistent with observations in these events on a small source size and weak, simple magnetic field configurations.

The fact that only  ${}^3\text{He}$  is observed above  $0.5\text{ MeV nucleon}^{-1}$  in the 2023 October 24 event could be due to its unique  $Q/M$  ratio ( $2/3$  for  ${}^3\text{He}^{+2}$ ) along with the small size of the jet where possibly only limited (wave) energy for ion acceleration is generated.  ${}^3\text{He}$ , with a unique  $Q/M$ , does not compete in absorbing wave energy with other ions and can spend a proportionally larger portion of available energy. Heavy ions in events #3–5 in Table 2 were also observed at low ( $<0.5\text{ MeV nucleon}^{-1}$ ) energies; however, these events have unknown solar sources. They all have  ${}^3\text{He}/{}^4\text{He}$  and  $\text{Fe}/\text{O}$  typical of  ${}^3\text{He}$ -rich events (G. M. Mason et al. 2002, 2016). Therefore, the examined event is special for its extreme  ${}^3\text{He}$  enrichment. Event #16 (highly enriched in  ${}^3\text{He}$ ) is the one in Table 2 whose heavy-ion spectra extend above  $\sim 1\text{ MeV nucleon}^{-1}$  (G. M. Mason et al. 2016). A weak photospheric magnetic field at the source of this event is a common feature with the 2023 October 24 event. However, event #16 showed a large, twisted jet (N. V. Nitta et al. 2015; D. E. Innes et al. 2016; G. M. Mason et al. 2016) with a projected size about 8

times greater than the straight jet in the October 24 event, supporting the idea about a possible connection between jet size/complexity and energy attained by heavy ions. Note that the base of the jet in both these events has a similar scale size and is located at the same angular distance from the center of the solar disk, implying a similar projection effect. Further supporting observations can be found in R. Bučik et al. (2018). The authors reported three  ${}^3\text{He}$ -rich SEP events having energy spectra of heavy ions extending beyond  $\sim 1\text{ MeV nucleon}^{-1}$  with sources at the CH edge associated with twisted and extremely elongated jets (projected length spanning  $40^\circ$ – $60^\circ$  of heliographic longitude). All jets were triggered by minifilament eruptions. The  ${}^3\text{He}/{}^4\text{He}$  and  $\text{Fe}/\text{O}$  ratios were  $\sim 1$ – $2$ . The heavy-ion enhancement patterns were not investigated in these events.

I. Roth & M. Temerin (1997) previously discussed the energization details of  ${}^3\text{He}$  and the heavy ions. The authors argued that heavy-ion energization can be significantly smaller because of their small acceleration rate. If the rate of ion acceleration is related to the jet, then a small and simple jet might not energize heavy ions efficiently. S. Liu et al. (2004, 2006) pointed to the faster acceleration of  ${}^3\text{He}$  (or, conversely, bigger losses for  ${}^4\text{He}$ ) that let  ${}^3\text{He}$  attain more energy. Since the losses are sensitive to temperature, the  ${}^4\text{He}$  acceleration is suppressed as temperature decreases (S. Liu et al. 2006). This leads to a decrease in  ${}^3\text{He}/{}^4\text{He}$  with increasing temperature. Fitting the energy spectra of  ${}^3\text{He}$  and  ${}^4\text{He}$ , the authors reported the temperature for events #1 and #2, which are listed in Table 2, as  $1.6$  and  $1.2\text{ MK}$ ,

**Table 2**  
Previously Reported  $^3\text{He}$ -rich SEP Events with Abundance Enhancement Pattern Not Ordered by Mass

| #   | SEP Start Date             | CH             | EUV Flare             |                       |                    | Minifilament     | Type III             | $^3\text{He}/^4\text{He}^m$ | $\log T^f$ (K) |
|-----|----------------------------|----------------|-----------------------|-----------------------|--------------------|------------------|----------------------|-----------------------------|----------------|
|     |                            |                | Type                  | Location              | Time               |                  |                      |                             |                |
| (1) | (2)                        | (3)            | (4)                   | (5)                   | (6)                | (7)              | (8)                  | (9)                         | (10)           |
| 1   | 1999-Mar-21 <sup>a</sup>   | Y <sup>b</sup> | Jet <sup>b</sup>      | N19W27 <sup>b</sup>   | 04:36 <sup>b</sup> | ? <sup>c</sup>   | ? <sup>c</sup>       | $3.65 \pm 0.15$             | ...            |
| 2   | 2000-Jan-06 <sup>a</sup>   | Y <sup>b</sup> | Ejection <sup>b</sup> | N15W52 <sup>b</sup>   | 02:36 <sup>b</sup> | ? <sup>c</sup>   | 02:03 <sup>c</sup>   | $23.42 \pm 4.69$            | ...            |
| 3   | 2000-Jan-09 <sup>a,d</sup> | ...            | ...                   | ...                   | ...                | ...              | 16:48 <sup>c,l</sup> | $0.29 \pm 0.02$             | ...            |
| 4   | 2000-Feb-02 <sup>d</sup>   | ...            | ...                   | ...                   | ...                | ...              | 09:45 <sup>c</sup>   | ...                         | ...            |
| 5   | 2001-Jul-16 <sup>a,d</sup> | ...            | ...                   | ...                   | ...                | ...              | 11:53 <sup>c</sup>   | $0.60 \pm 0.09$             | ...            |
| 6   | 2002-Apr-05 <sup>a</sup>   | ...            | ...                   | ...                   | ...                | ...              | 20:42 <sup>c,l</sup> | $0.05 \pm 0.01$             | ...            |
| 7   | 2002-Sep-25 <sup>a</sup>   | ...            | ...                   | ...                   | ...                | ...              | 18:42 <sup>c,l</sup> | $2.33 \pm 0.46$             | ...            |
| 8   | 2002-Oct-20 <sup>a</sup>   | Y <sup>b</sup> | Jet <sup>b</sup>      | S16W60 <sup>b</sup>   | 14:24 <sup>b</sup> | ? <sup>c</sup>   | 14:11 <sup>c</sup>   | $1.35 \pm 0.04$             | ...            |
| 9   | 2002-Oct-21 <sup>a</sup>   | Y <sup>b</sup> | Jet <sup>b</sup>      | S16W68 <sup>b</sup>   | 04:24 <sup>b</sup> | ? <sup>c</sup>   | 04:17 <sup>c</sup>   | $1.28 \pm 0.05$             | ...            |
| 10  | 2003-Apr-28 <sup>a</sup>   | ...            | ...                   | ...                   | ...                | ...              | 04:01 <sup>c</sup>   | $0.22 \pm 0.02$             | ...            |
| 11  | 2011-Jul-9 <sup>a</sup>    | Y <sup>c</sup> | Jet <sup>c</sup>      | N14W44 <sup>c</sup>   | 16:25 <sup>c</sup> | Y <sup>c</sup>   | 16:25 <sup>c,l</sup> | $5.21 \pm 0.49$             | 6.36           |
| 12  | 2012-Aug-02 <sup>a</sup>   | N <sup>c</sup> | Jet <sup>f</sup>      | N12W58 <sup>f</sup>   | 03:00 <sup>f</sup> | Y <sup>f</sup>   | 03:00 <sup>f</sup>   | $0.45 \pm 0.02$             | 6.32           |
| 13  | 2012-Nov-20 <sup>a</sup>   | N <sup>c</sup> | Jet <sup>g,h</sup>    | S17W60 <sup>g,h</sup> | 01:31 <sup>g</sup> | Y <sup>c</sup>   | 01:30 <sup>g,h</sup> | $7.66 \pm 0.87$             | 6.31           |
| 14  | 2014-Apr-17 <sup>a</sup>   | N <sup>c</sup> | Eruption <sup>g</sup> | S15W24 <sup>g</sup>   | 21:50 <sup>g</sup> | Y <sup>c</sup>   | 21:58 <sup>g</sup>   | $0.61 \pm 0.04$             | 6.54           |
| 15  | 2014-Apr-24 <sup>a</sup>   | Y <sup>c</sup> | Eruption <sup>g</sup> | S18W102 <sup>g</sup>  | 00:50 <sup>g</sup> | Y <sup>c</sup>   | 00:40 <sup>g</sup>   | $1.13 \pm 0.06$             | ...            |
| 16  | 2014-May-16 <sup>a</sup>   | Y <sup>g</sup> | Jet <sup>g</sup>      | S12W44 <sup>g</sup>   | 04:02 <sup>c</sup> | Y <sup>a,i</sup> | 03:57 <sup>g</sup>   | $14.88 \pm 1.36$            | 6.31           |
| 17  | 2015-Feb-06 <sup>a</sup>   | N <sup>c</sup> | Jet <sup>f</sup>      | N14W19 <sup>f</sup>   | 23:31 <sup>c</sup> | Y <sup>c</sup>   | 23:30 <sup>f,l</sup> | $1.76 \pm 0.28$             | 6.19           |
| 18  | 2022-Mar-06 <sup>j</sup>   | N <sup>c</sup> | Jet <sup>j</sup>      | W26S16 <sup>j</sup>   | 23:55 <sup>c</sup> | Y <sup>j</sup>   | 23:55 <sup>j,l</sup> | $0.97 \pm 0.02$             | ...            |
| 19  | 2023-Apr-08 <sup>k</sup>   | ...            | ...                   | ...                   | ...                | ...              | ...                  | $5.50 \pm 0.30$             | ...            |

**Notes.**<sup>a</sup> Event in G. M. Mason et al. (2016).<sup>b</sup> Y. M. Wang et al. (2006).<sup>c</sup> This work.<sup>d</sup> Event in G. M. Mason et al. (2002).<sup>e</sup> R. Bučik et al. (2014).<sup>f</sup> R. Bučik et al. (2021).<sup>g</sup> N. V. Nitta et al. (2015).<sup>h</sup> N.-H. Chen et al. (2015).<sup>i</sup> D. E. Innes et al. (2016).<sup>j</sup> Event in R. Bučik et al. (2023).<sup>k</sup> Event in G. M. Mason et al. (2023).<sup>l</sup> Day before SEP start date.<sup>m</sup> #1–3, #5–17 at 0.5–2.0 MeV nucleon<sup>-1</sup> and #18–19 at 0.320–0.452 MeV nucleon<sup>-1</sup>.

respectively. These temperatures are similar to the temperature of the examined event. G. M. Mason et al. (2024) suggested that the huge  $^3\text{He}/^4\text{He}$  ratios are due to a combination of the higher energy achieved by  $^3\text{He}$  along with a rollover in the spectrum at high energies.

The examined event showed a decline in  $^4\text{He}$ . D. V. Reames (2019a) reported rare  $^4\text{He}$ -poor events among  $^3\text{He}$ -rich events with abundances  $^4\text{He}/\text{O} < 30$ . The author discussed that in a model of the FIP effect,  $^4\text{He}$ , with its unique high FIP value (24.6 eV), is slowly ionized in transit to the corona (J. M. Laming 2009), leading to its suppression by a factor of 2. D. V. Reames (2019b) speculated that the observed sufficient  $^4\text{He}$  suppression may occur if the transition is fast, e.g., in jets. G. C. Ho et al. (2019) reported four out of a 100  $^3\text{He}$ -rich events with no  $^4\text{He}$  intensity increase above the background at  $\sim 1$  MeV nucleon<sup>-1</sup> (though  $^4\text{He}$  could be present at lower energies).

### 3.3. Temperature and Heavy-ion Elemental Composition in the 2023 October 24 Event

Typical  $^3\text{He}$ -rich events show an enhancement pattern that increases approximately as a power law with  $Q/M$  (e.g., Figure 9 in G. M. Mason et al. 2004). Perhaps these S-peaked events have more wave activity but less reconnection, since

reconnection produces power laws (J. F. Drake et al. 2009). Models of  $^3\text{He}$ -rich SEP heating and acceleration by plasma waves (L. A. Fisk 1978; M. Temerin & I. Roth 1992) have been previously used to discuss temperature and elemental abundances (e.g., I. Roth & M. Temerin 1997; G. M. Mason et al. 1980, 2023). We estimate heavy-ion abundances, applying for the first time the EM-derived temperatures for the given solar source, in the models of L. A. Fisk (1978) and I. Roth & M. Temerin (1997).

In the L. A. Fisk (1978) model,  $^3\text{He}$  enrichment is achieved through heating by electrostatic ion cyclotron waves excited in the frequency range near the  $^3\text{He}$  gyrofrequency (i.e., between the  $^4\text{He}^{+2}$  and H cyclotron frequencies).  $^4\text{He}^{+2}$  and H are also heated, but their thermal speeds are significantly lower than  $^3\text{He}^{+2}$ . Heavy ions, partially stripped of their electrons, have a second harmonic of their gyrofrequency in the same frequency range as  $^3\text{He}$  and can be heated too. For example,  $^{24}\text{Mg}$  with eight electrons removed has the second harmonic of its gyrofrequency equal to the  $^3\text{He}$  gyrofrequency. The wave excitation requires relatively high  $\text{He}/\text{H}$  ( $\gtrsim 0.2$ ), a low ( $< 10^{-3}$ ) plasma  $\beta$ , and a ratio of electron to ion temperature  $T_e/T_i < 10$ . Heated ions are then injected into the (unspecified) flare-acceleration process. Based on the model of L. A. Fisk (1978), Figure 11(a) shows the fractions of the ionization states of



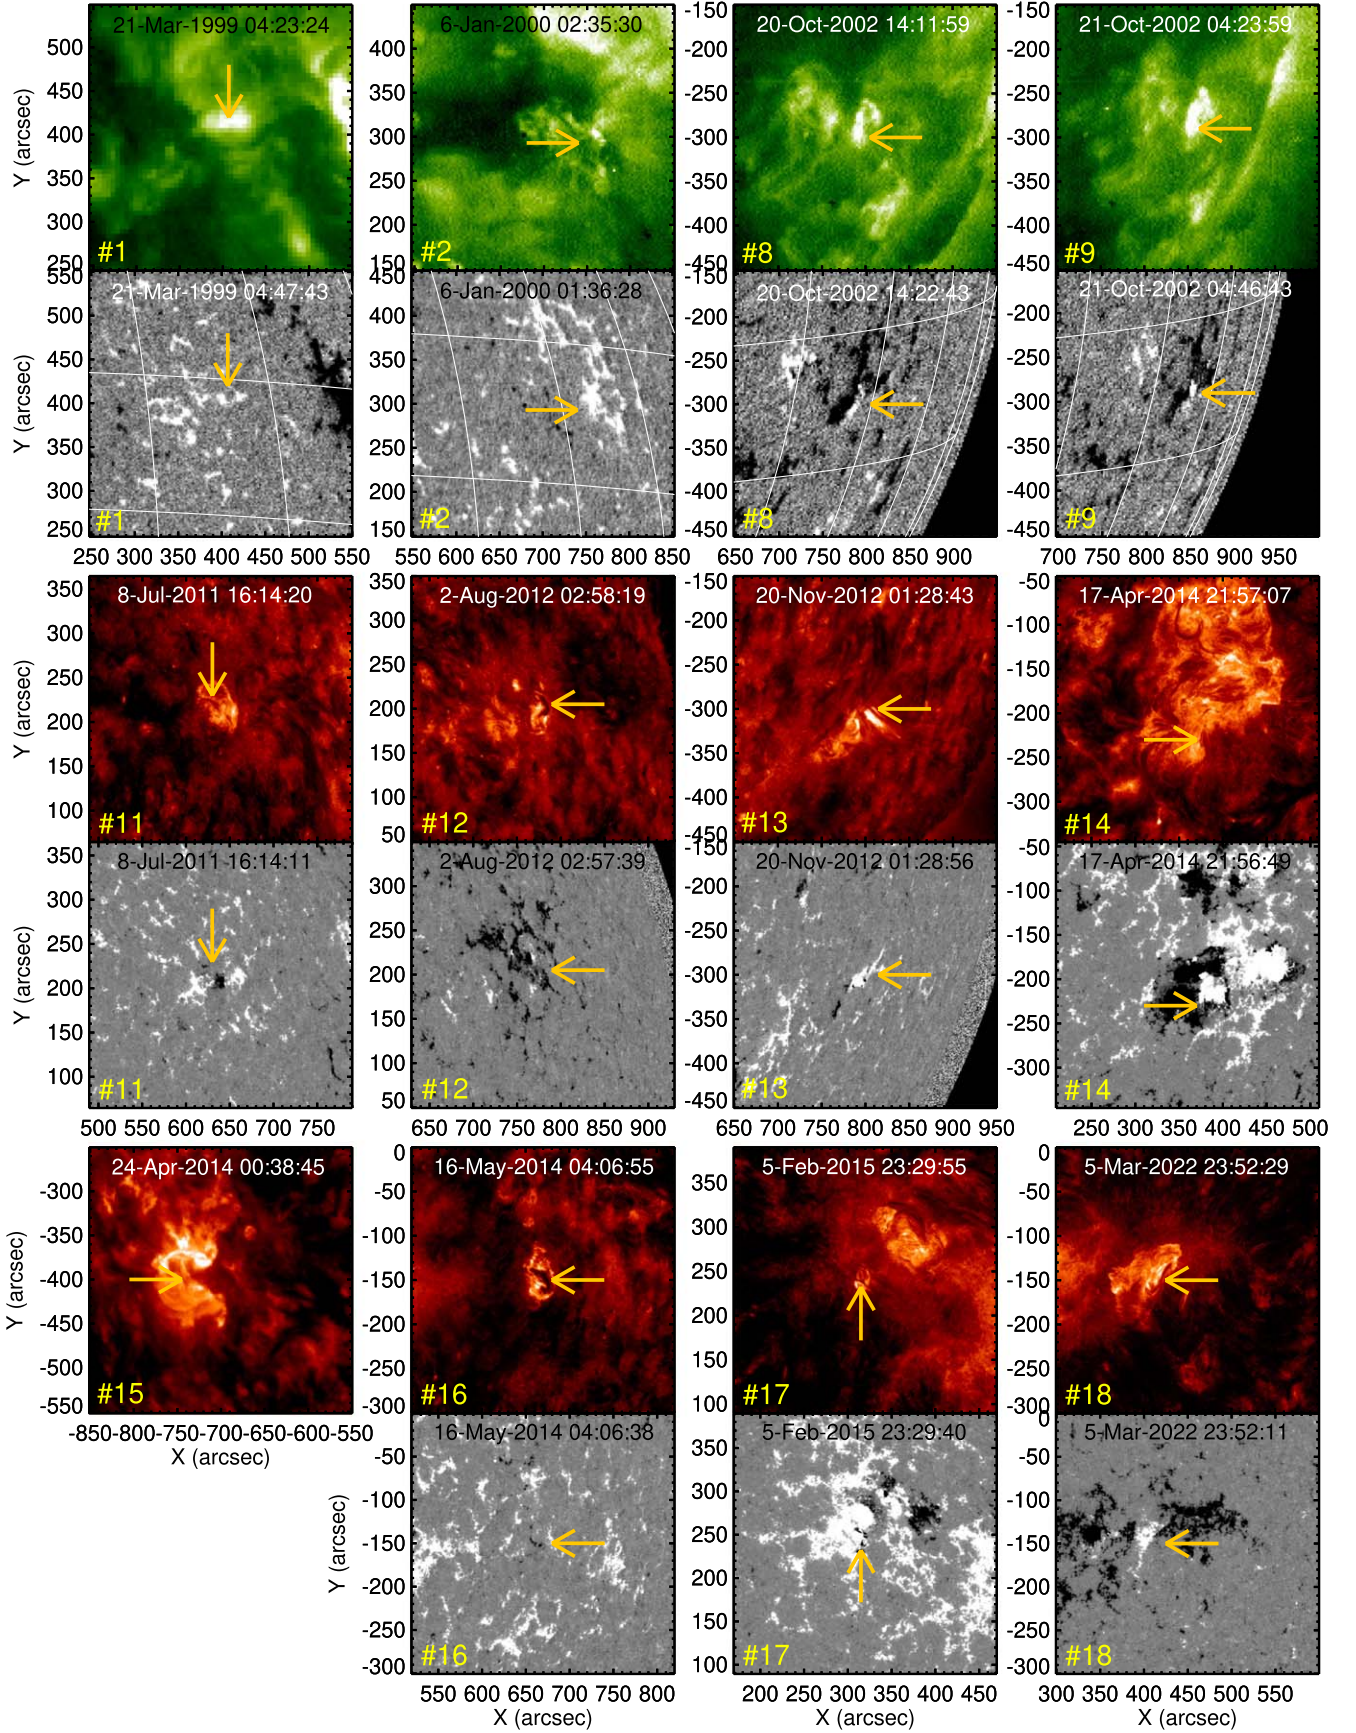

**Figure 10.** Solar sources of events #1–2 and #8–9 in EIT 195 Å images and MDI magnetograms. For these events, arrows mark EUV flare location from Table 2 (column (5)). Solar sources of events #11–14 and #16–17 in AIA 304 Å images and HMI magnetograms. Solar source of event #15 in EUVI 304 Å. For events #11–18, arrows mark the locations of erupting minifilaments.

selected ion species that fall within the limits given by formula (6) in G. M. Mason et al. (1980) as a function of temperature, assuming the most recent equilibrium charge states from the CHIANTI atomic database (K. P. Dere et al. 1997; G. Del Zanna et al. 2021) and the relative isotopic abundances given by K. Lodders (2003). Formula (6), repeated below from G. M. Mason et al. (1980), gives the frequency range for which species  $i$  will be resonantly heated:

$$1.05 < 2\Omega_i/\Omega_{\text{He}} < 1.19 + 0.13(m_{\text{He}}/m_i)^{1/2}, \quad (1)$$

where  $\Omega_i$  is the gyrofrequency, and  $m_i$ , and  $m_{\text{He}}$  are the masses of the ion and  ${}^4\text{He}$ , respectively. It shows the lower and upper bound frequencies for the ion second harmonics, given in units of  ${}^4\text{He}$  gyrofrequency. The formula was derived from the minimum critical electron speed required to excite electrostatic ion cyclotron waves. A lower bound of 1.05 ensures  $T_e/T_i < 10$ . The upper bound was obtained for  $T_e/T_i = 5$ , the value where  ${}^3\text{He}$  is effectively heated, as discussed by L. A. Fisk (1978). Note that  ${}^{12}\text{C}$  does not have gyrofrequencies in the range of frequencies for preferential heating given by Equation (1). Only the minor isotope  ${}^{13}\text{C}$  (and with  $Q = +4$ ) contributes, which has an abundance of 1% of  ${}^{12}\text{C}$  (K. Lodders 2003).

M. Temerin & I. Roth (1992) and I. Roth & M. Temerin (1997) proposed a model of direct acceleration (where no heating is required) of  ${}^3\text{He}^{+2}$  by electromagnetic cyclotron waves that propagate with frequency between the H and  ${}^4\text{He}^{+2}$  gyrofrequencies. The abundant species H and  ${}^4\text{He}^{+2}$  are not accelerated because of cyclotron damping of the waves. Heavy species with  $Q/M < 0.5$  are accelerated at the second or higher harmonics of their cyclotron frequency. Contrary to the model of L. A. Fisk (1978), here a wide range of gyrofrequencies is available for acceleration. Figure 11(b) shows the fractions of the ionization states of selected ion species with  $Q/M < 0.49$ , i.e., those that fall below the damped-wave region. I. Roth & M. Temerin (1997) noted that the heavier ions are more likely to have a charge-to-mass ratio of less than 0.50 (see also Figure 7 in G. M. Mason et al. 2023), and thus are more likely to be accelerated. Furthermore, the authors pointed out that thermal heavy ions can be removed from resonance by Coulomb collisions whose rate is equivalent to  $Q^2/M$ .

Figure 11(c) plots the spatially averaged EM curves in a rectangle surrounding the solar source at different times. The EM curve peaks at  $\log T$  (K) = 6.1 ( $\sim 1.3$  MK) at 19:47 UT,  $\log T$  (K) = 6.2 ( $\sim 1.6$  MK) at 19:48 UT (time of minifilament eruption), and  $\log T$  (K) = 6.3 ( $\sim 2$  MK) at 19:49/19:50 UT (time of type III burst). The source region is multithermal, as suggested by the broad distribution of EM curves. The broadening is most obvious around type III radio burst time. For example, at 19:49 UT, there is 0.3 MK plasma in the source with a factor of  $\sim 3$  lower EM than the peak (2 MK) temperature. At the same time, there is also a  $\sim 20$  MK component with an EM a factor of  $>10$  lower than the peak (2 MK) temperature.

Using EM-determined temperature, we estimate the fractional abundances of ions for preferential heating or acceleration in the 2023 October 24 event. The dominant temperature (i.e., temperature with maximum EM) would not be a good choice as this neglects other temperatures at the source. We may select fractional abundances at EM-weighted temperatures. However, a single temperature, even when EM-weighted, does not reflect fractional abundance profiles with temperature.

Fractional abundances at various temperatures should be considered as the plasma in the source is multithermal. Therefore, we multiply EM (normalized to the area under the EM curve) with fractional abundance curves shown in Figures 11(a) and (b). The integral of this multiplication over the temperature range yields the average fractional abundance. For the EM at 19:49 UT and fractional abundances in Figure 11(a), the average fractional abundances in percent are 0.24 (C), 0.44 (N), 2.20 (O), 3.36 (Ne), 5.46 (Mg), 12.1 (Si), 17.0 (S), 23.2 (Ca), and 18.5 (Fe). The values obtained from Figure 11(b) are 40.1 (C), 66.4 (N), 85.2 (O), 95.3 (Ne), 97.1 (Mg), 97.9 (Si), 99.2 (S), and 100 (Ca–Fe).

We apply these average fractional abundances to the recommended solar corona composition reported by J. T. Schmelz et al. (2012) to estimate the abundances of heated or accelerated populations. We normalized the average fractional abundances to O and multiplied them with solar corona abundances, which were also normalized to O. Figure 12 shows the derived abundances at 19:48, 19:49, and 19:50 UT from fractions in the two models in Figures 11(a) and (b) and, for comparison, the  $0.193 \text{ MeV nucleon}^{-1}$  2023 October 24 event abundances. The comparison is adequate for low-energy ions where charge states depend only on temperature (e.g., L. Kocharov et al. 2000) and not on charge-stripping effects causing the energy dependence of heavy-ion charge states observed in  ${}^3\text{He}$ -rich events at higher energies,  $\sim 0.2\text{--}1 \text{ MeV nucleon}^{-1}$  (e.g., B. Klecker et al. 2007; R. DiFabio et al. 2008). Overplotted in Figure 12 are  $0.386 \text{ MeV nucleon}^{-1}$   ${}^3\text{He}$ -rich SEP (G. M. Mason et al. 2004) and solar corona values. The average fractional abundance of N cannot be correctly determined from the fractions in Figure 11(a) as the N curve is located mostly below the minimum EM-derived temperature. Thus, the abundance of N could be treated as underestimated. For the same reason, the abundance of O is also partially affected.

### 3.3.1. Fisk Model

Figure 12 shows that the pattern of heavy-ion (Ne–Ca) abundances estimated from fractions in the L. A. Fisk (1978) model (Figure 11(a)) is consistent with measurements, with a peak at Si. Within uncertainties, the estimated abundances at the minifilament eruption (19:48 UT) agree with the observed abundances. Thus, the specific EM distribution of temperatures could be one cause of the unusual heavy-ion abundance enhancement pattern. Around the time of the type III radio burst (19:49–19:50 UT), the pattern remains preserved, but the estimated abundances decrease, and Ne and Mg approach typical  ${}^3\text{He}$ -rich SEP values. This may raise the question of whether enhanced composition was produced early in the solar event, before type III burst onset. The Fe/O in the examined event is consistent with the solar corona value and is well below the typical  ${}^3\text{He}$ -rich SEP and the estimated ratio. This may suggest that Fe is not preferentially heated, though the average fractional abundance of Fe is the second highest among other species. The high abundance of C would be hard to reproduce with its maximum fractional abundance of  $\sim 1\%$  (see Figure 11(a)), and therefore remains puzzling.

### 3.3.2. Roth and Temerin Model

Figure 12 shows that the red curves, the estimated relative abundances from fractions in the model of I. Roth & M. Temerin (1997; see Figure 11(b)), all lie almost on top of each other.



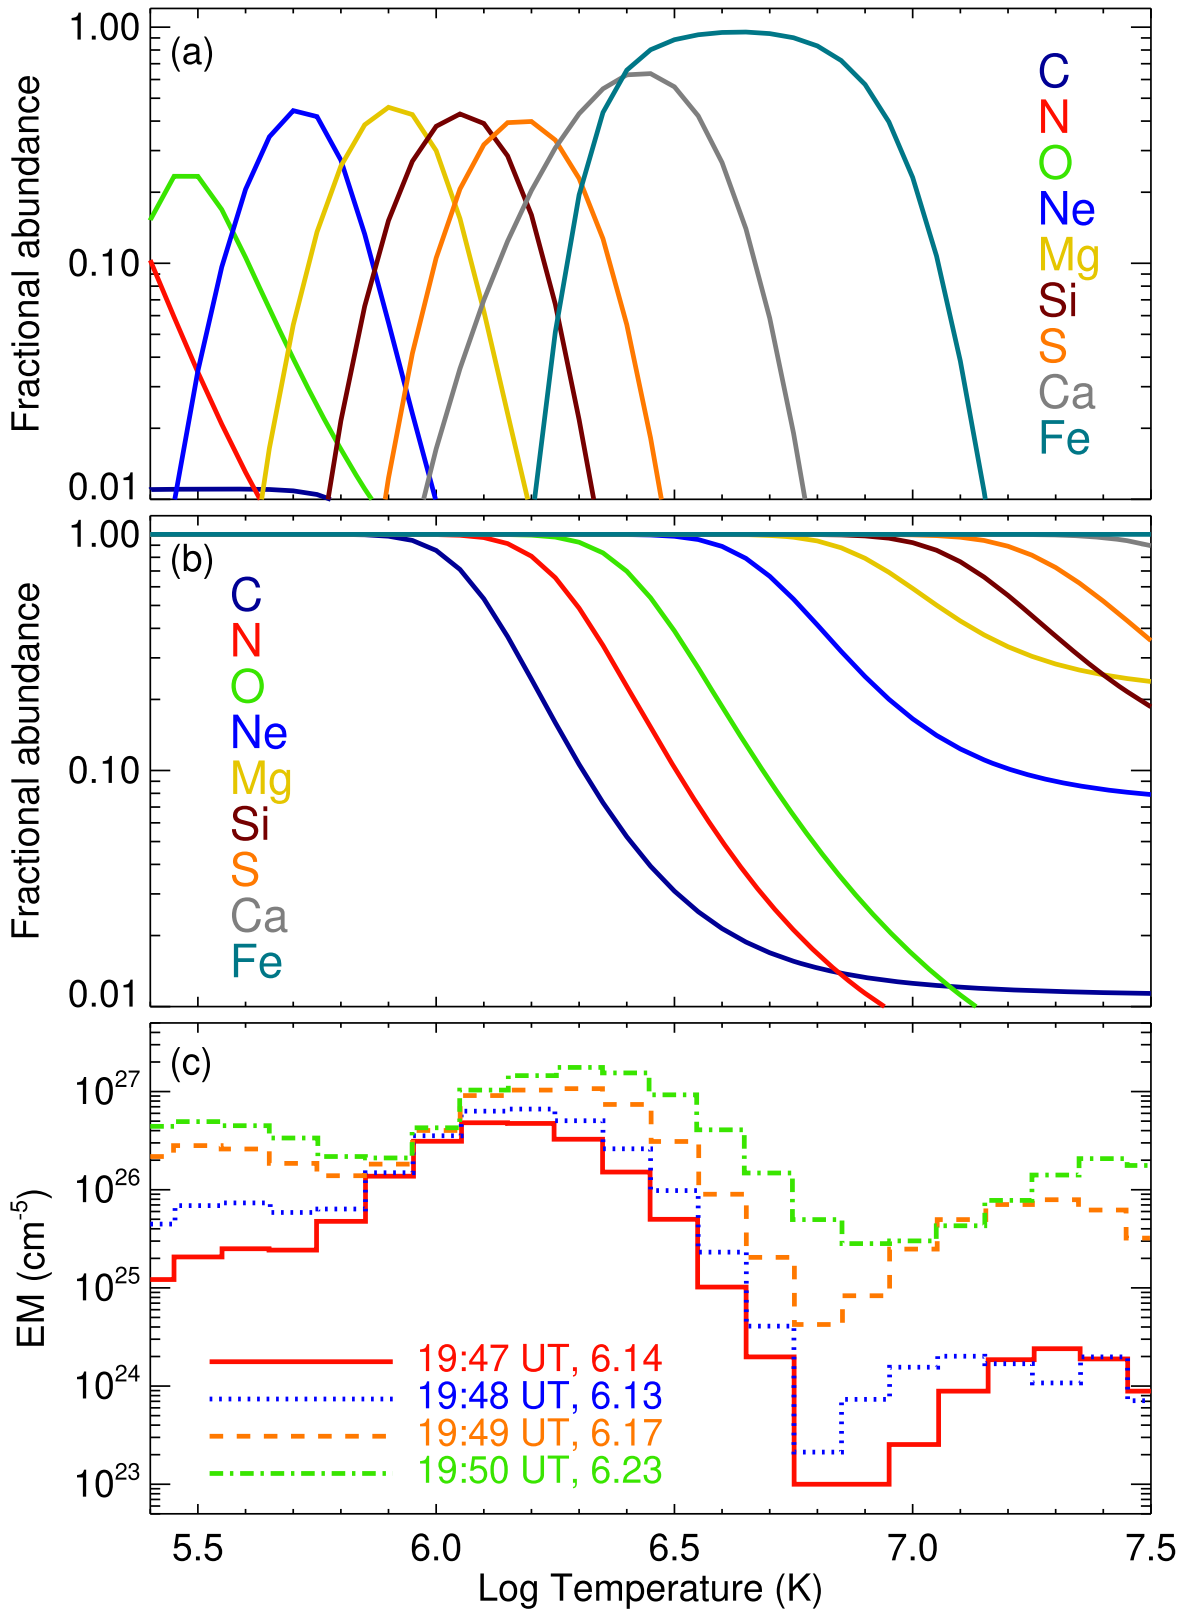

**Figure 11.** (a) Fractional abundance of selected heavy-ion species whose gyrofrequency falls in the range of preferential heating given by Equation (1) as a function of equilibrium temperature (after G. M. Mason et al. 1980). (b) Fractional abundance of selected heavy-ion species whose  $Q/M$  falls below the damped-wave region (after G. M. Mason et al. 2023) as a function of equilibrium temperature. (c) The EM profiles in the solar source (spatially averaged in the white rectangle in Figure 8) at the start time of the event-associated type III radio burst (19:50 UT) and three other times preceding the type III burst. The EM-weighted log temperatures in kelvin are shown for these four times.



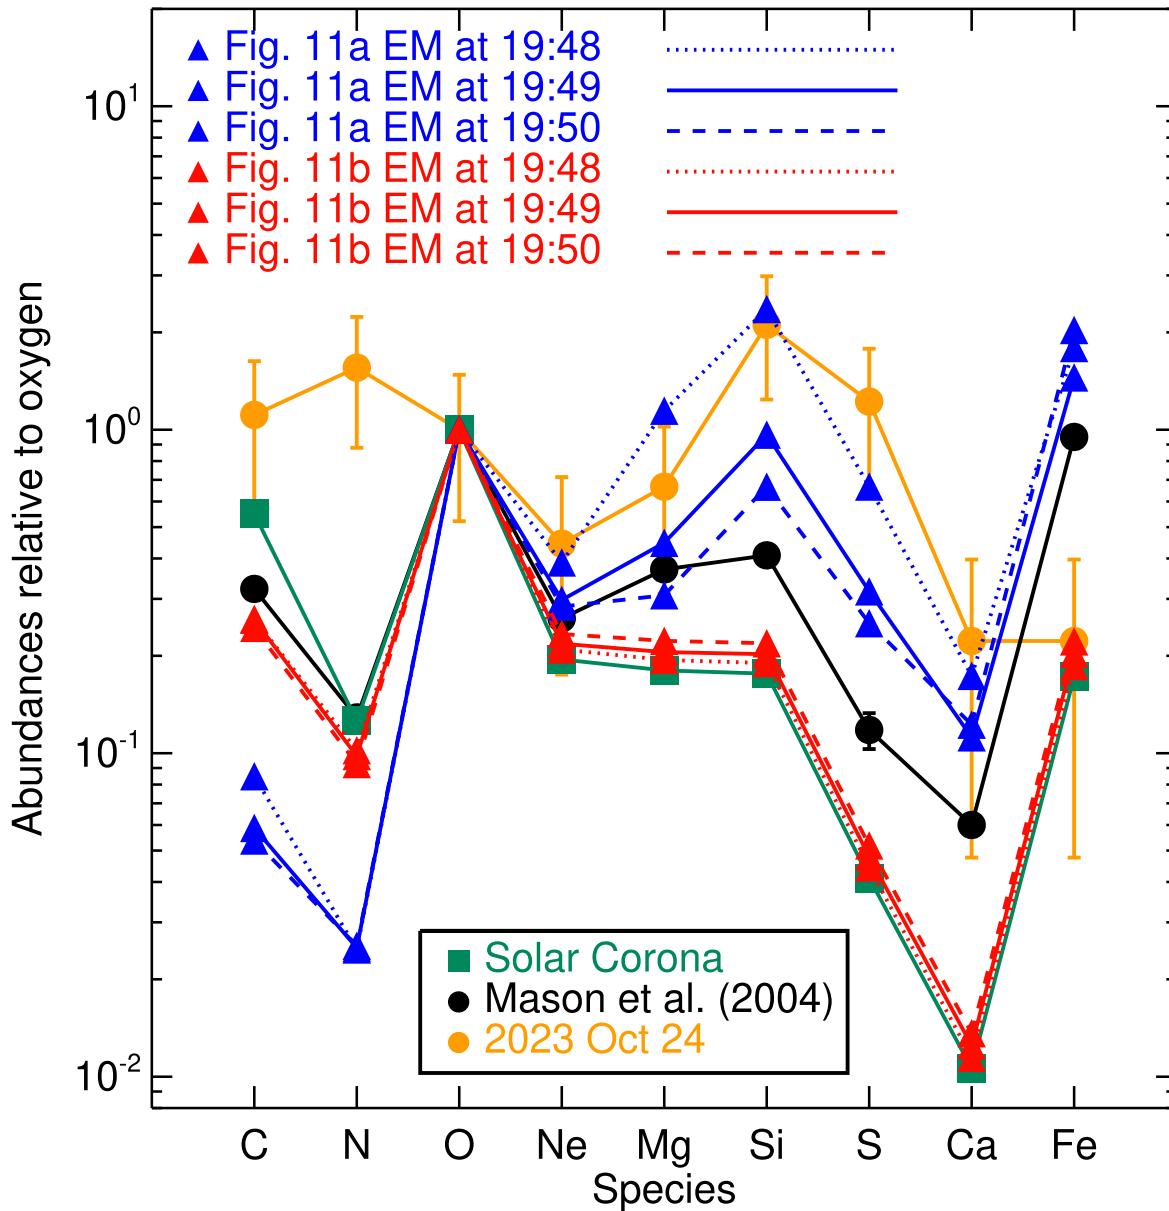

**Figure 12.** Estimated abundances from fractions in models in Figure 11, using the EM at 19:48 (dotted lines), 19:49 (solid lines), 19:50 UT (dashed lines), and solar corona abundances. Overplotted are  $0.193 \text{ MeV nucleon}^{-1}$  2023 October 24 event,  $0.386 \text{ MeV nucleon}^{-1}$   $^3\text{He}$ -rich SEP (G. M. Mason et al. 2004), and solar corona (J. T. Schmelz et al. 2012) abundances.

Except for C (and partially N), the red lines lie close to the solar corona values. This is because the average abundance fractions of heavy-ion species are close or equal to each other (i.e., all ions participate equally), placing the abundances relative to O at unity. Thus, the temperature (or its EM distribution) in the examined source could not produce the required abundances in the I. Roth & M. Temerin (1997) model. However, a hot source, where the average fractional abundances of heavier ions decrease, would create an enhancement in the relative abundance of Ne–Fe, similar to those obtained from the L. A. Fisk (1978) model.

The fractional abundance of C is below or equal to O for  $\log T \lesssim 7.1$  ( $\sim 12.6 \text{ MK}$ ; see Figure 11(b)), implying that the relative fractional abundance of C could be as high as unity (at a cooler source). However, above that temperature, the fractional abundance of C relative to O is greater than 1 but less than  $\sim 3$  (not visible in Figure 11(b)). This can easily cause

a great enhancement of C above typical  $^3\text{He}$ -rich SEP values. Below  $\log T \lesssim 5.9$  ( $\sim 0.8 \text{ MK}$ ; see Figure 11(b)), where the fractional abundance of C is 1, only faint relative enhancement of C above a typical  $^3\text{He}$ -rich SEP value can be produced. For N, the threshold temperature is  $\log T \lesssim 7.4$  ( $\sim 25 \text{ MK}$ ; not shown), where the fractional abundance of N relative to O is slightly above 1, but  $\lesssim 1.5$ . This can hardly lead to an enhancement of N above the typical  $^3\text{He}$ -rich SEP value from a baseline coronal composition. Below  $\log T \lesssim 6.1$  ( $\sim 1.3 \text{ MK}$ ; see Figure 11(b)), where the fractional abundance of N is 1, the relative abundance of N would not exceed the typical  $^3\text{He}$ -rich SEP value.

The above discussion suggests that high temperatures are required to produce abundance enhancement in the I. Roth & M. Temerin (1997) model. For example, ions could be accelerated only at a certain altitude at the source where the temperature is high, though the spatially averaged EM is low.

Using a spatially averaged EM is a simplification. Maybe ions are accelerated in spots within the source region, where EM peaks at high temperatures. In both these cases, the I. Roth & M. Temerin (1997) model could be adequate for the examined event. Sites with a hot temperature (e.g., with an EM peaking at  $\sim 10$  MK) would produce enhancement of heavier species (Ne–Fe) and C. This idea is consistent with G. M. Mason et al. (2023) suggestion that heavy-ion enhancement is mainly due to O depletion at high temperatures in the I. Roth & M. Temerin (1997) model.

The emphasis on temperature affecting the ion  $Q/M$ , followed by many earlier works, may not be central in the heating and acceleration of  $^3\text{He}$ -rich SEPs. In this case, it might be that the puzzling enhancement pattern of heavy ions does not require a special temperature or temperature range. G. M. Mason & B. Klecker (2018) suggested a mechanism that is sensitive to temperature, but where heavy-ion enhancement is due to their lower ionization losses after the passage of a small amount of material. The combined stochastic acceleration with Coulomb losses has been suggested for the enrichment of heavy and ultraheavy ions by Y. Y. Kartavykh et al. (2020). The model by S. Liu et al. (2006), developed for  $^3\text{He}$  and  $^4\text{He}$ , does not require any special temperature considerations of the type called for by L. A. Fisk (1978) or I. Roth & M. Temerin (1997).

The spectral forms in the S. Liu et al. (2006) model produce  $^3\text{He}/^4\text{He}$  ratios that vary greatly with energy, which may explain the lack of correlation of Fe and  $^3\text{He}$  enrichments (G. M. Mason et al. 1986; D. V. Reames et al. 1994), which are not addressed by the L. A. Fisk (1978) or I. Roth & M. Temerin (1997) models (see R. M. Winglee 1989). In the region of high-energy spectral rollover, models such as those by S. Liu et al. (2006) can in principle produce extreme  $^3\text{He}/^4\text{He}$  ratios such as shown in Figure 4.

#### 4. Conclusion

Below, we summarize key observational features of the  $^3\text{He}$ -rich SEP event measured at 0.47 au by Solar Orbiter on 2023 October 24.

1. An odd ion enhancement pattern, not ordered by mass, with high abundances of C, and particularly N, Si, and S, and with depleted  $^4\text{He}$  and Fe.
2. The energy spectra of all heavy ions except  $^3\text{He}$  were measured below  $\sim 0.5$  MeV nucleon $^{-1}$ .
3.  $^3\text{He}/^4\text{He}$  increasing with energy, attaining an extreme value not observed in previous events.
4. A solar source with supergranulation scale size, characterized by a weak photospheric field at the edge of a CH, where a minifilament eruption triggered a faint straight jet.

The presented results suggest that the EM temperature distribution at the solar source could be one factor that affects the selection of ion species for preferential heating and acceleration. A simplified concept of EM spatially averaged at the source reproduces the observed abundance pattern for the 2023 October 24 event with the L. A. Fisk (1978) model for Ne–Ca, but C, N, and Fe do not fit into the observed abundance pattern. For the I. Roth & M. Temerin (1997) model, acceleration in sites with high temperatures would be required. The enhancement of N remains puzzling in this model.

The addition of similar  $^3\text{He}$ -rich SEP events with abundances not ordered by mass indicates that cool minifilaments may be a common feature of such events. However, it is unclear whether the cool material of minifilaments plays a role, as it would not be needed for the I. Roth & M. Temerin (1997) model. The energy achieved by heavy ions seems to be influenced by the size and shape of jets in these events. Finally, strong photospheric fields at the source of these events are not needed for extreme  $^3\text{He}$  enrichments.

$^3\text{He}$ -rich SEP events where heavy-ion enrichments are not ordered by mass are rare. Probably they are too small at 1 au to be measured above  $\sim 0.5$ –1 MeV nucleon $^{-1}$ . Thus, Solar Orbiter at closer distances to  $^3\text{He}$ -rich solar sources enables us to detect such events at higher energies and even those weak events that were missed at 1 au. Understanding these events is necessary for a more complete picture of the ion heating/acceleration of  $^3\text{He}$ -rich SEPs.

#### Acknowledgments

R.B. acknowledges support by NASA grant Nos. 80NSSC21K1316 and 80NSSC22K0757. S.M.M. acknowledges support from the UK Research and Innovation's Science and Technology Facilities Council under grant award numbers ST/T000422/1 and ST/X000990/1. Solar Orbiter is a mission of international cooperation between ESA and NASA, operated by ESA. The Suprathermal Ion Spectrograph (SIS) is a European facility instrument funded by ESA under contract number SOL.ASTR.CON.00004 with CAU. We thank ESA and NASA for their support of the Solar Orbiter and other missions whose data were used in this paper. Solar Orbiter post-launch work at JHU/APL and the Southwest Research Institute is supported by NASA contract NNN06AA01C and at CAU by German Space Agency (DLR) grant No. 50OT2002. The UAH team acknowledges financial support by the Spanish Ministerio de Ciencia, Innovación y Universidades MCIU/AEI Project PID2019 – 104863RBI00/AEI/10.13039/501100011033. CHIANTI is a collaborative project involving George Mason University (USA), the University of Michigan (USA), the University of Cambridge (UK), and NASA Goddard Space Flight Center (USA). This study benefited from discussions within the International Space Science Institute (ISSI) Team ID 425 Origins of  $^3\text{He}$ -rich SEPs that concluded in 2022.

#### ORCID iDs

Radoslav Bučík 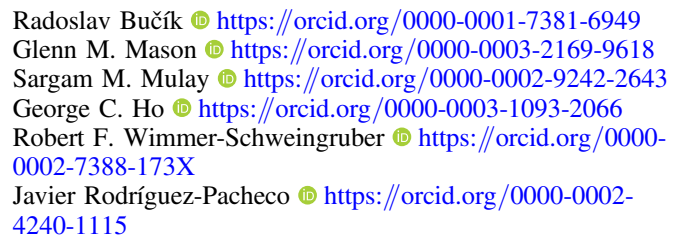 <https://orcid.org/0000-0001-7381-6949>  
 Glenn M. Mason 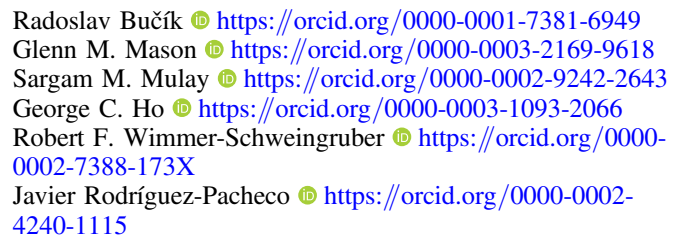 <https://orcid.org/0000-0003-2169-9618>  
 Sargam M. Mulay 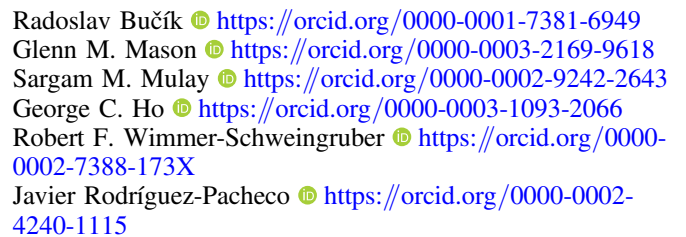 <https://orcid.org/0000-0002-9242-2643>  
 George C. Ho 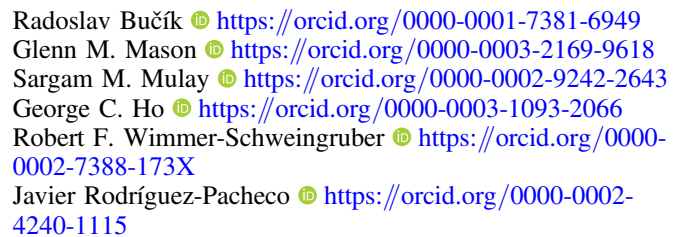 <https://orcid.org/0000-0003-1093-2066>  
 Robert F. Wimmer-Schweingruber 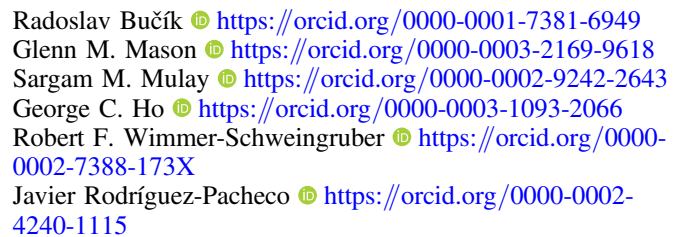 <https://orcid.org/0000-0002-7388-173X>  
 Javier Rodríguez-Pacheco 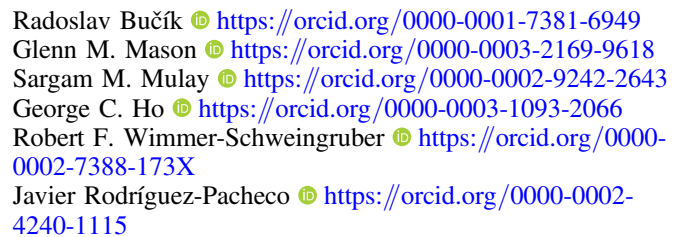 <https://orcid.org/0000-0002-4240-1115>

#### References

- Bale, S. D., Goetz, K., Harvey, P. R., et al. 2016, *SSRv*, **204**, 49  
 Bodmer, R., Bochsler, P., Geiss, J., von Steiger, R., & Gloeckler, G. 1995, *SSRv*, **72**, 61  
 Bougeret, J. L., Goetz, K., Kaiser, M. L., et al. 2008, *SSRv*, **136**, 487  
 Bougeret, J. L., Kaiser, M. L., Kellogg, P. J., et al. 1995, *SSRv*, **71**, 231  
 Burlaga, L. F. 1995, *Interplanetary Magnetohydrodynamics* (Oxford: Oxford Univ. Press)  
 Bučík, R. 2020, *SSRv*, **216**, 24

- Bučík, R., Innes, D. E., Mall, U., et al. 2014, [ApJ](#), **786**, 71
- Bučík, R., Innes, D. E., Mason, G. M., et al. 2018, [ApJ](#), **852**, 76
- Bučík, R., Mall, U., Korth, A., & Mason, G. M. 2009, [AnGeo](#), **27**, 3677
- Bučík, R., Mason, G. M., Nitta, N. V., et al. 2023, [A&A](#), **673**, L5
- Bučík, R., Mulay, S. M., Mason, G. M., et al. 2021, [ApJ](#), **908**, 243
- Chen, N.-H., Bučík, R., Innes, D. E., & Mason, G. M. 2015, [A&A](#), **580**, A16
- Cheung, M. C. M., Boerner, P., Schrijver, C. J., et al. 2015, [ApJ](#), **807**, 143
- Delaboudinière, J. P., Artzner, G. E., Brunaud, J., et al. 1995, [SoPh](#), **162**, 291
- Del Zanna, G. 2013, [A&A](#), **558**, A73
- Del Zanna, G., Dere, K. P., Young, P. R., & Landi, E. 2021, [ApJ](#), **909**, 38
- Del Zanna, G., O'Dwyer, B., & Mason, H. E. 2011, [A&A](#), **535**, A46
- De Pontieu, B., Title, A. M., Lemen, J. R., et al. 2014, [SoPh](#), **289**, 2733
- Dere, K. P., Del Zanna, G., Young, P. R., Landi, E., & Sutherland, R. S. 2019, [ApJS](#), **241**, 22
- Dere, K. P., Landi, E., Mason, H. E., Monsignori Fossi, B. C., & Young, P. R. 1997, [A&AS](#), **125**, 149
- DiFabio, R., Guo, Z., Möbius, E., et al. 2008, [ApJ](#), **687**, 623
- Drake, J. F., Cassak, P. A., Shay, M. A., Swisdak, M., & Quataert, E. 2009, [ApJL](#), **700**, L16
- Ebert, R. W., Dayeh, M. A., Desai, M. I., & Mason, G. M. 2012, [ApJ](#), **749**, 73
- Fisk, L. A. 1978, [ApJ](#), **224**, 1048
- Freeland, S. L., & Handy, B. N. 1998, [SoPh](#), **182**, 497
- Gloeckler, G., & Geiss, J. 1998, [SSRv](#), **84**, 275
- Hart, S. T., Dayeh, M. A., Bučík, R., et al. 2022, [ApJS](#), **263**, 22
- Heinemann, S. G., Temmer, M., Heinemann, N., et al. 2019, [SoPh](#), **294**, 144
- Hill, M. E., Mitchell, D. G., Andrews, G. B., et al. 2017, [JGR](#), **122**, 1513
- Ho, G. C., Mason, G. M., & Allen, R. C. 2019, [SoPh](#), **294**, 33
- Horbury, T. S., O'Brien, H., Carrasco Blazquez, I., et al. 2020, [A&A](#), **642**, A9
- Howard, R. A., Moses, J. D., Vourlidas, A., et al. 2008, [SSRv](#), **136**, 67
- Innes, D. E., Bučík, R., Guo, L. J., & Nitta, N. 2016, [AN](#), **337**, 1024
- Kartavykh, Y. Y., Dröge, W., Klecker, B., Kovaltsov, G. A., & Ostryakov, V. M. 2020, [ApJ](#), **888**, 48
- Klecker, B., Möbius, E., & Popecki, M. A. 2007, [SSRv](#), **130**, 273
- Kocharov, L., Kovaltsov, G. A., Torsti, J., & Ostryakov, V. M. 2000, [A&A](#), **357**, 716
- Laming, J. M. 2009, [ApJ](#), **695**, 954
- Laming, J. M., & Kuroda, N. 2023, [ApJ](#), **951**, 86
- Lemen, J. R., Title, A. M., Akin, D. J., et al. 2012, [SoPh](#), **275**, 17
- Liu, S., Petrosian, V., & Mason, G. M. 2004, [ApJL](#), **613**, L81
- Liu, S., Petrosian, V., & Mason, G. M. 2006, [ApJ](#), **636**, 462
- Lodders, K. 2003, [ApJ](#), **591**, 1220
- Maksimovic, M., Bale, S. D., Chust, T., et al. 2020, [A&A](#), **642**, A12
- Mason, G. M. 2007, [SSRv](#), **130**, 231
- Mason, G. M., Dwyer, J. R., & Mazur, J. E. 2000, [ApJL](#), **545**, L157
- Mason, G. M., Gloeckler, G., Fisk, L. A., & Hovestadt, D. 1980, [ApJ](#), **239**, 1070
- Mason, G. M., & Klecker, B. 2018, [ApJ](#), **862**, 7
- Mason, G. M., Kouloumvakos, A., Ho, G. C., et al. 2024, [ApJ](#), **974**, 54
- Mason, G. M., Leske, R. A., Desai, M. I., et al. 2008, [ApJ](#), **678**, 1458
- Mason, G. M., Mazur, J. E., & Dwyer, J. R. 2002, [ApJL](#), **565**, L51
- Mason, G. M., Mazur, J. E., Dwyer, J. R., et al. 2004, [ApJ](#), **606**, 555
- Mason, G. M., Nitta, N. V., Wiedenbeck, M. E., & Innes, D. E. 2016, [ApJ](#), **823**, 138
- Mason, G. M., Reames, D. V., Klecker, B., Hovestadt, D., & von Rosenvinge, T. T. 1986, [ApJ](#), **303**, 849
- Mason, G. M., Roth, I., Nitta, N. V., et al. 2023, [ApJ](#), **957**, 112
- Müller, D., St. Cyr, O. C., Zouganelis, I., et al. 2020, [A&A](#), **642**, A1
- Nitta, N. V., Mason, G. M., Wang, L., Cohen, C. M. S., & Wiedenbeck, M. E. 2015, [ApJ](#), **806**, 235
- O'Dwyer, B., Del Zanna, G., Mason, H. E., Weber, M. A., & Tripathi, D. 2010, [A&A](#), **521**, A21
- Owen, C. J., Bruno, R., Livi, S., et al. 2020, [A&A](#), **642**, A16
- Panesar, N. K., Sterling, A. C., Moore, R. L., & Chakrapani, P. 2016, [ApJL](#), **832**, L7
- Reames, D. V. 1995, [AdSpR](#), **15**, 41
- Reames, D. V. 2019a, [SoPh](#), **294**, 37
- Reames, D. V. 2019b, [SoPh](#), **294**, 141
- Reames, D. V. 2021a, *Solar Energetic Particles* (Cham: Springer)
- Reames, D. V. 2021b, [FrASS](#), **8**, 164
- Reames, D. V. 2002, [ApJL](#), **571**, L63
- Reames, D. V. 2023, [Univ](#), **9**, 466
- Reames, D. V., Cliver, E. W., & Kahler, S. W. 2014, [SoPh](#), **289**, 3817
- Reames, D. V., Meyer, J. P., & von Rosenvinge, T. T. 1994, [ApJS](#), **90**, 649
- Reames, D. V., & Ng, C. K. 2004, [ApJ](#), **610**, 510
- Reames, D. V., Richardson, I. G., & Barbier, L. M. 1991, [ApJL](#), **382**, L43
- Rieutord, M., & Rincon, F. 2010, [LRSP](#), **7**, 2
- Rochus, P., Auchère, F., Berghmans, D., et al. 2020, [A&A](#), **642**, A8
- Rodríguez-Pacheco, J., Wimmer-Schweingruber, R. F., Mason, G. M., et al. 2020, [A&A](#), **642**, A7
- Roth, I., & Temerin, M. 1997, [ApJ](#), **477**, 940
- Scherrer, P. H., Bogart, R. S., Bush, R. I., et al. 1995, [SoPh](#), **162**, 129
- Scherrer, P. H., Schou, J., Bush, R. I., et al. 2012, [SoPh](#), **275**, 207
- Schmelz, J. T., Reames, D. V., von Steiger, R., & Basu, S. 2012, [ApJ](#), **755**, 33
- Schrijver, C. J., & De Rosa, M. L. 2003, [SoPh](#), **212**, 165
- Sterling, A. C., Moore, R. L., Falconer, D. A., et al. 2016, [ApJ](#), **821**, 100
- Temerin, M., & Roth, I. 1992, [ApJL](#), **391**, L105
- Wang, Y. M., Pick, M., & Mason, G. M. 2006, [ApJ](#), **639**, 495
- Winglee, R. M. 1989, [ApJ](#), **343**, 511
